# Supplementary material for: Interpretation of the apparent activation energy of glass transition
Source: arXiv:2012.07264 source file (2020-12-14)

# Analysis of Viscosity of Glasses

K. Shirai

30 Aug. 2020

# Silica Glasses

# Soda-lime-silica glass

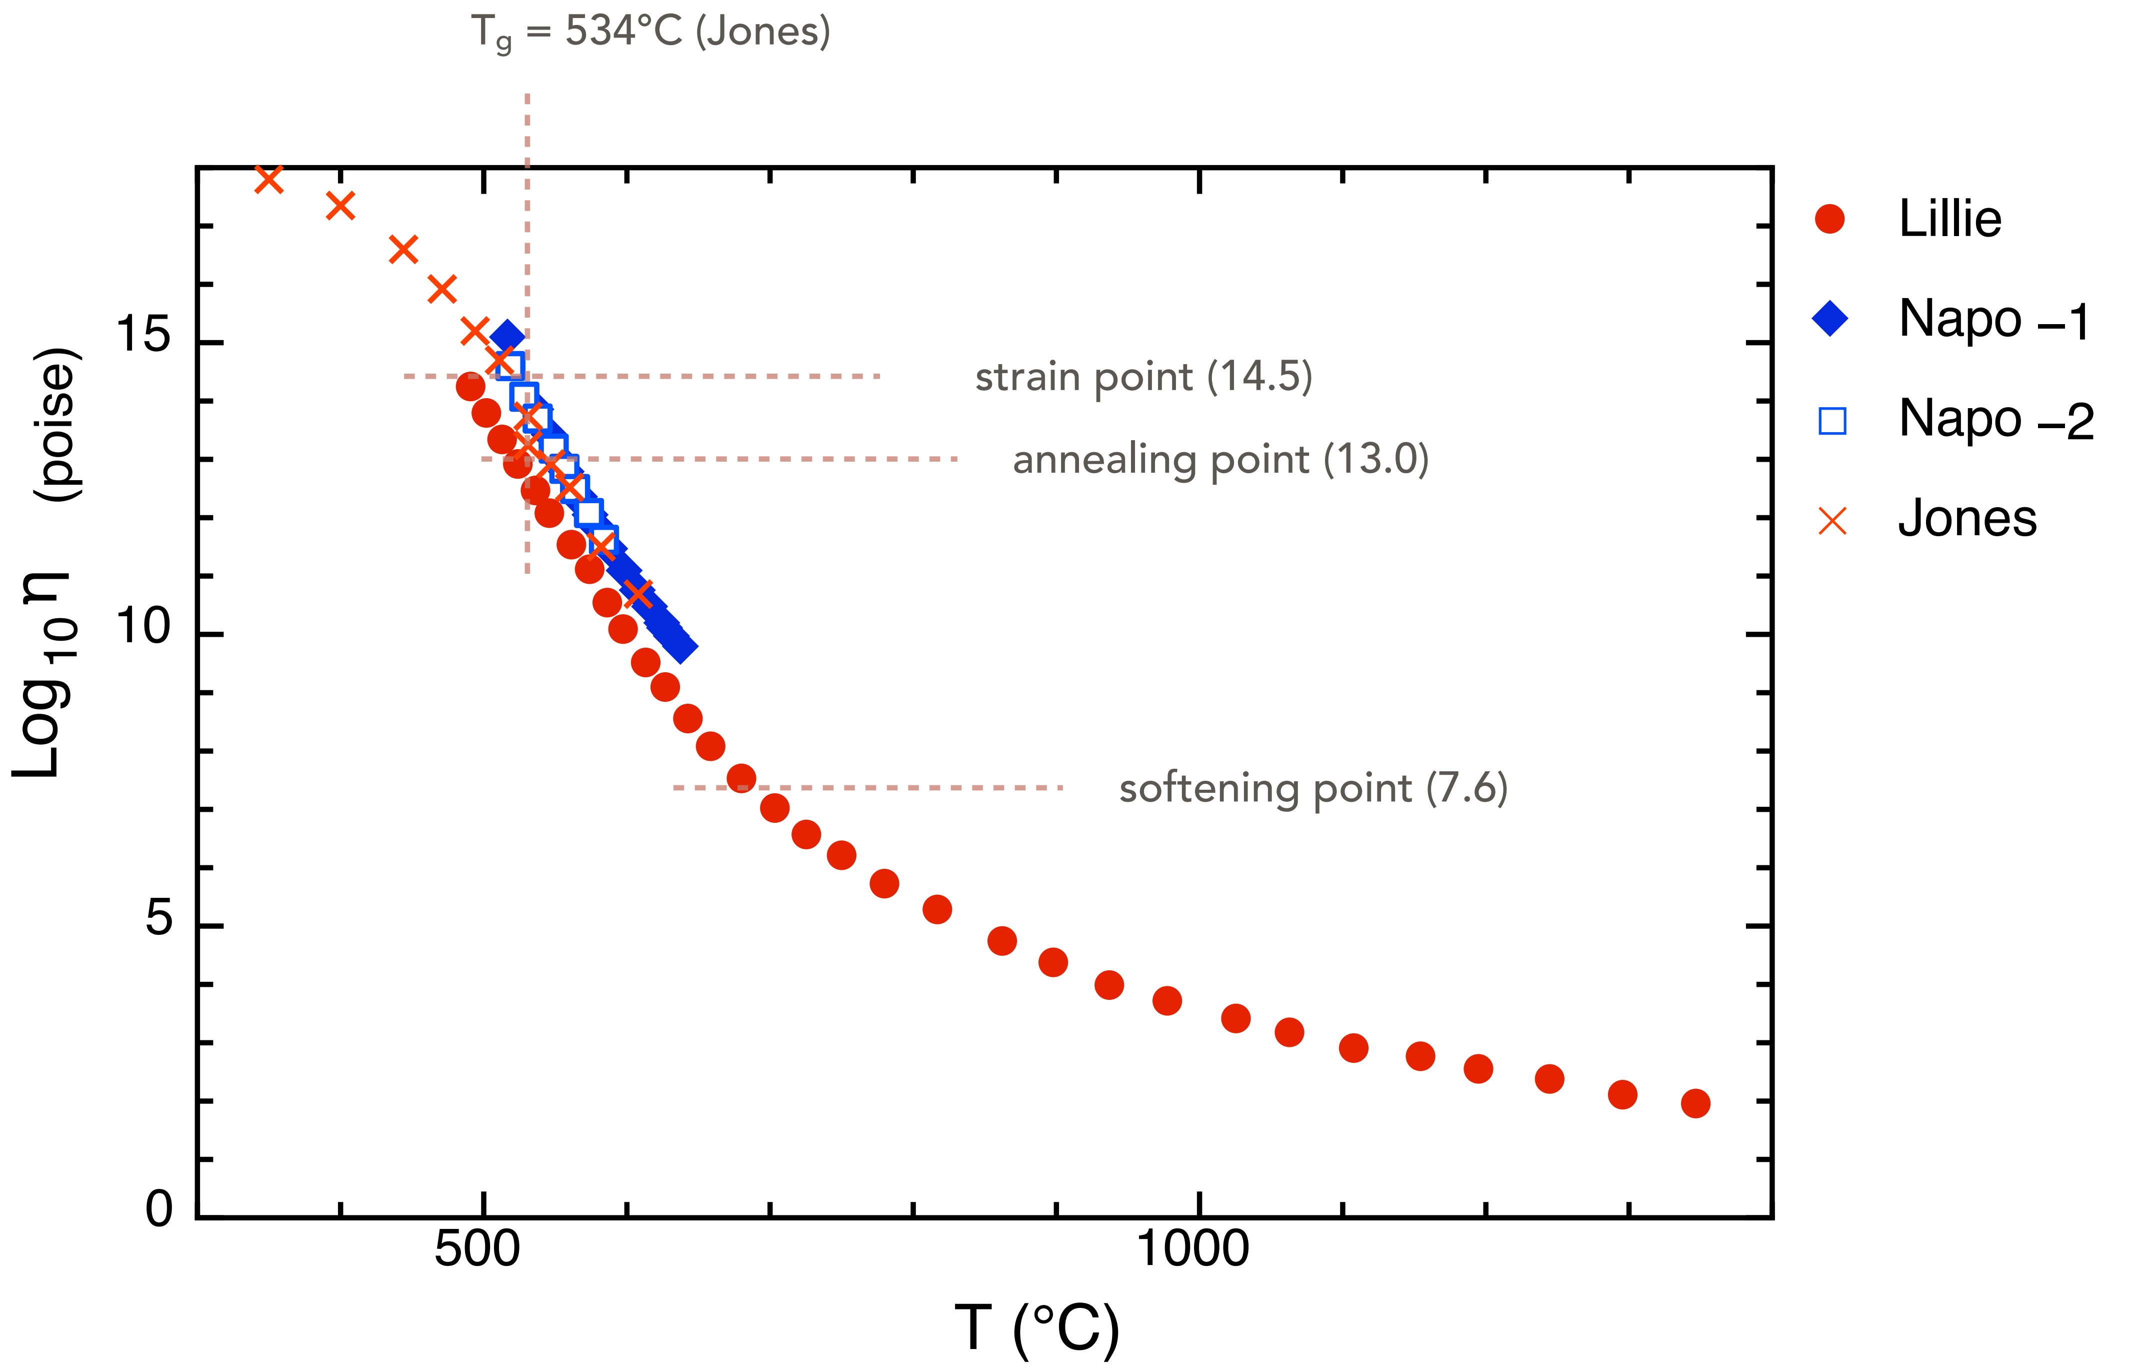



G. O. Jones, Rep. Prog. Phys. **12**, 133 (1949)

H. R. Lillie, J. Amer. Ceram. Soc. **14**, 502 (1931)

Napolitano and E. G. Hawkins, J. Res. Natl. Bur. Stand. **68**A, 439 (1964)

# Jones

G. O. Jones, Rep. Prog. Phys. **12**, 133 (1949)

Tg = 534°C

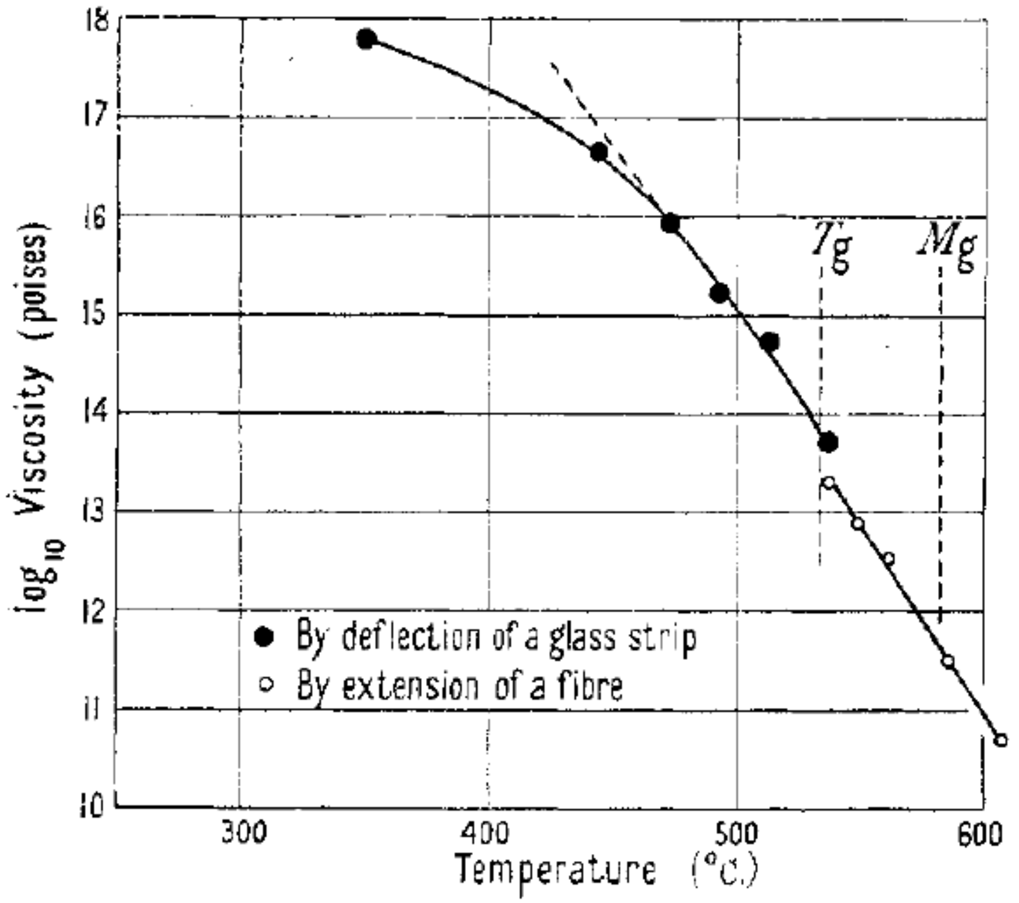


If the calculation of the activation energy for viscous flow is extended to these values of viscosity below the transition region, the striking result is obtained that its value falls off with decreasing temperature.

Q : 55 → 6 kcal/mol

2.3 → 0.25 eV

Originally
G. O. Jones, J. Soc. Glass Tech. **28**, 432 (1944)

# Jones

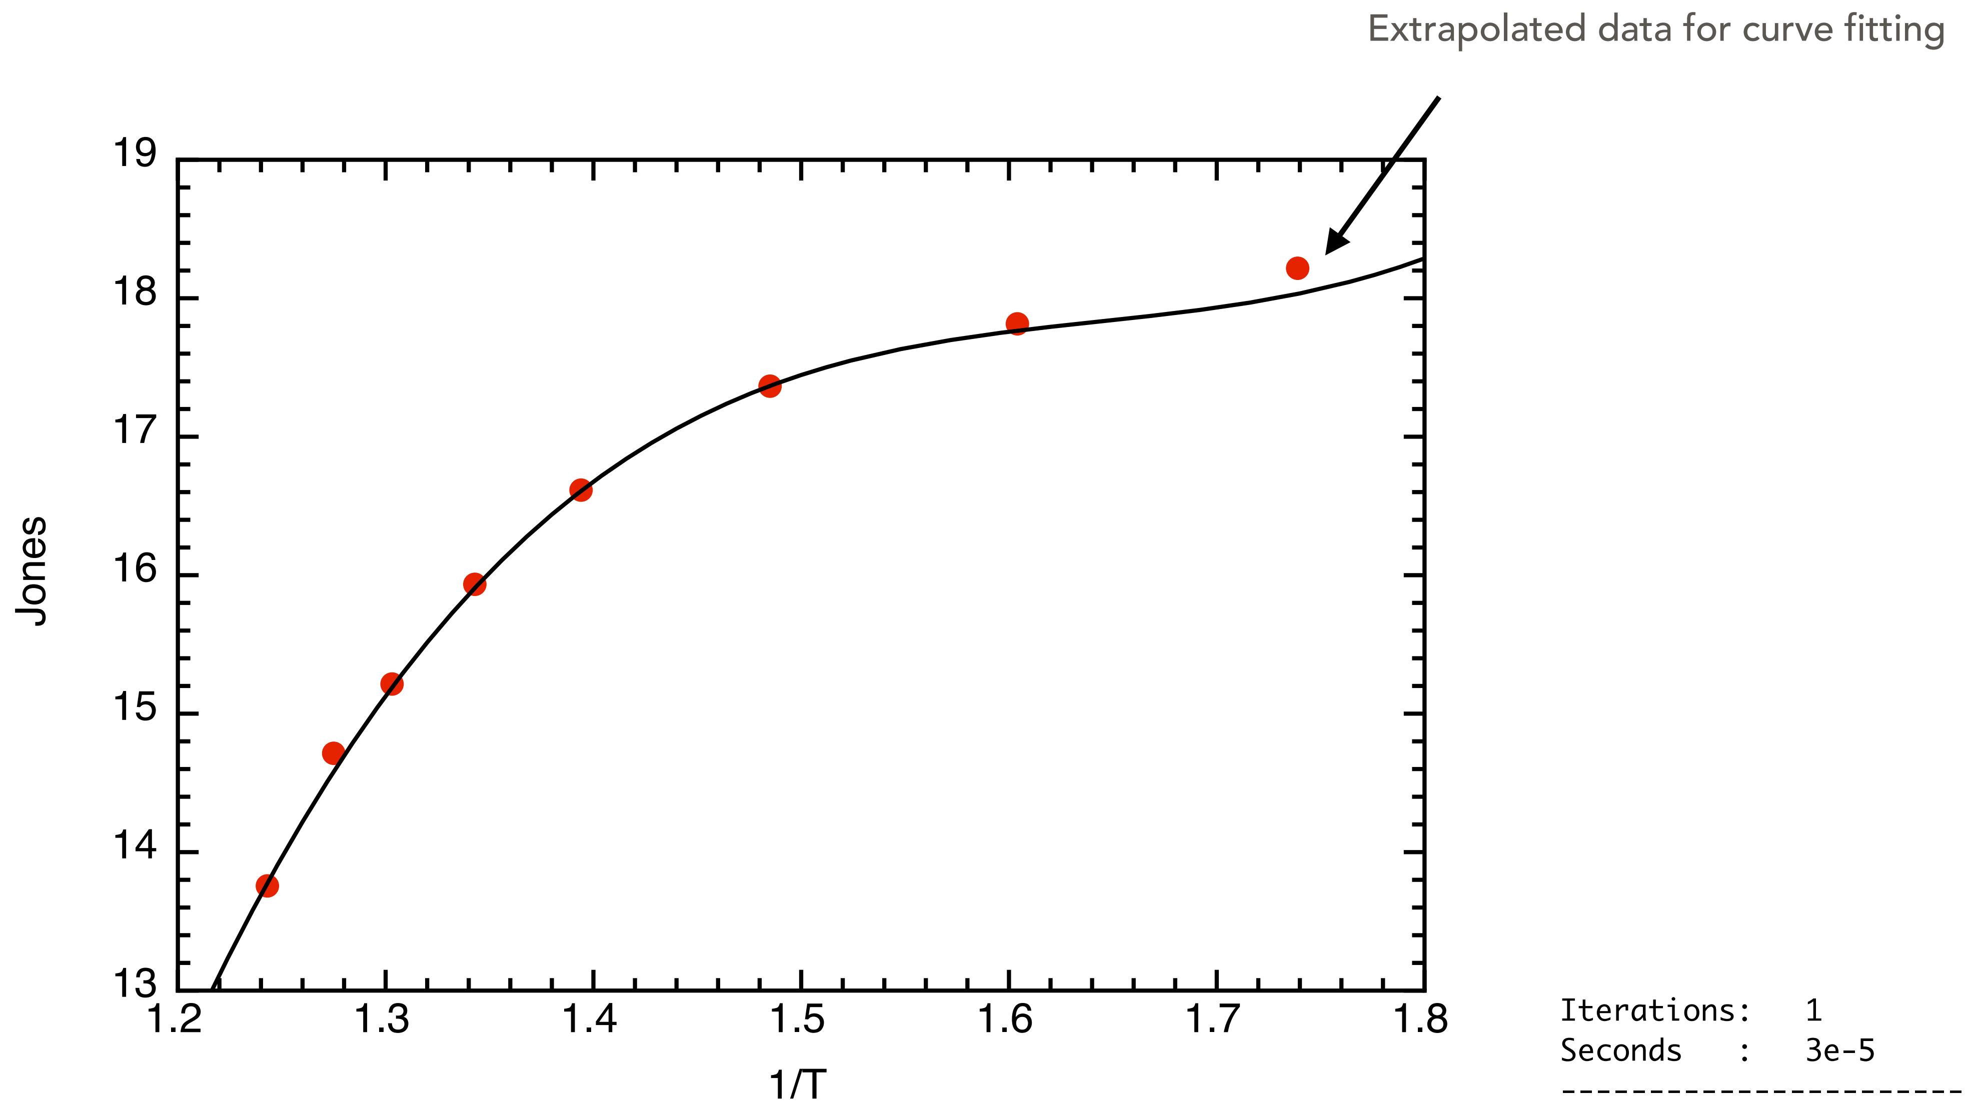


```
Iterations:   1
Seconds    :  3e-5
-------------------------------------------
Chi squared          =      0.012851

Parameters:                            Standard deviations:
deg     =        3.0000
const   =     -237.3304     Δconst =      22.4338
a1      =      467.8980     Δa1    =      45.7661
a2      =     -287.4441     Δa2    =      30.9242
a3      =       59.1604     Δa3    =       6.9200

Coefficient of Determination :            0.9993
Mean value of y-values y[i]  :            16.1887
Sum of squares of y[i]-yMean :            17.4215
Sum of squares of residuals  :            0.012851
```

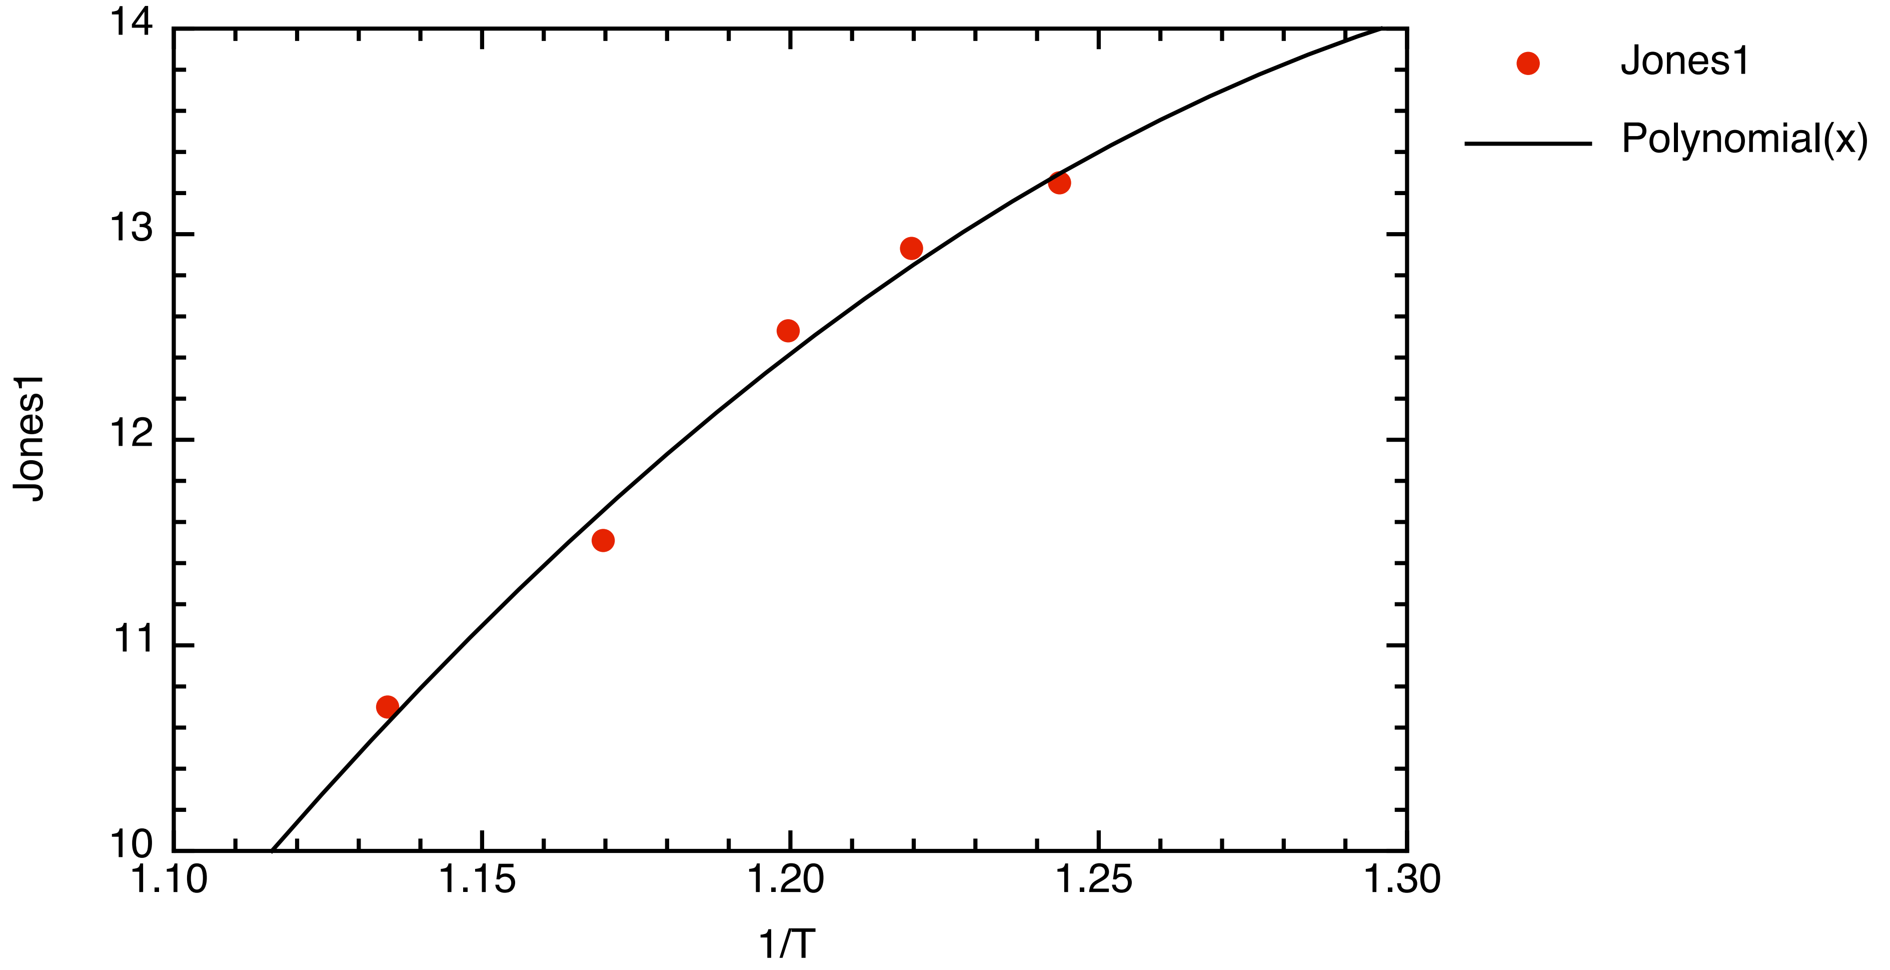


```
Iterations:   1
Seconds   :   4.6e-5
-------------------------------------------
Chi squared          =      0.049356

Parameters:                           Standard deviations:
deg     =         2.0000
const   =      -113.1445      Δconst =       79.3603
a1      =       186.2310      Δa1    =      133.6095
a2      =       -67.9961      Δa2    =       56.1877

Coefficient of Determination :            0.9890
Mean value of y-values y[i]  :            12.1740
Sum of squares of y[i]-yMean :            4.4691
Sum of squares of residuals  :            0.049356
```

# Lillie

T_soften = 670°C
T_strain = 479°C

H. R. Lillie, J. Amer. Ceram. Soc. **14**, 502 (1931)

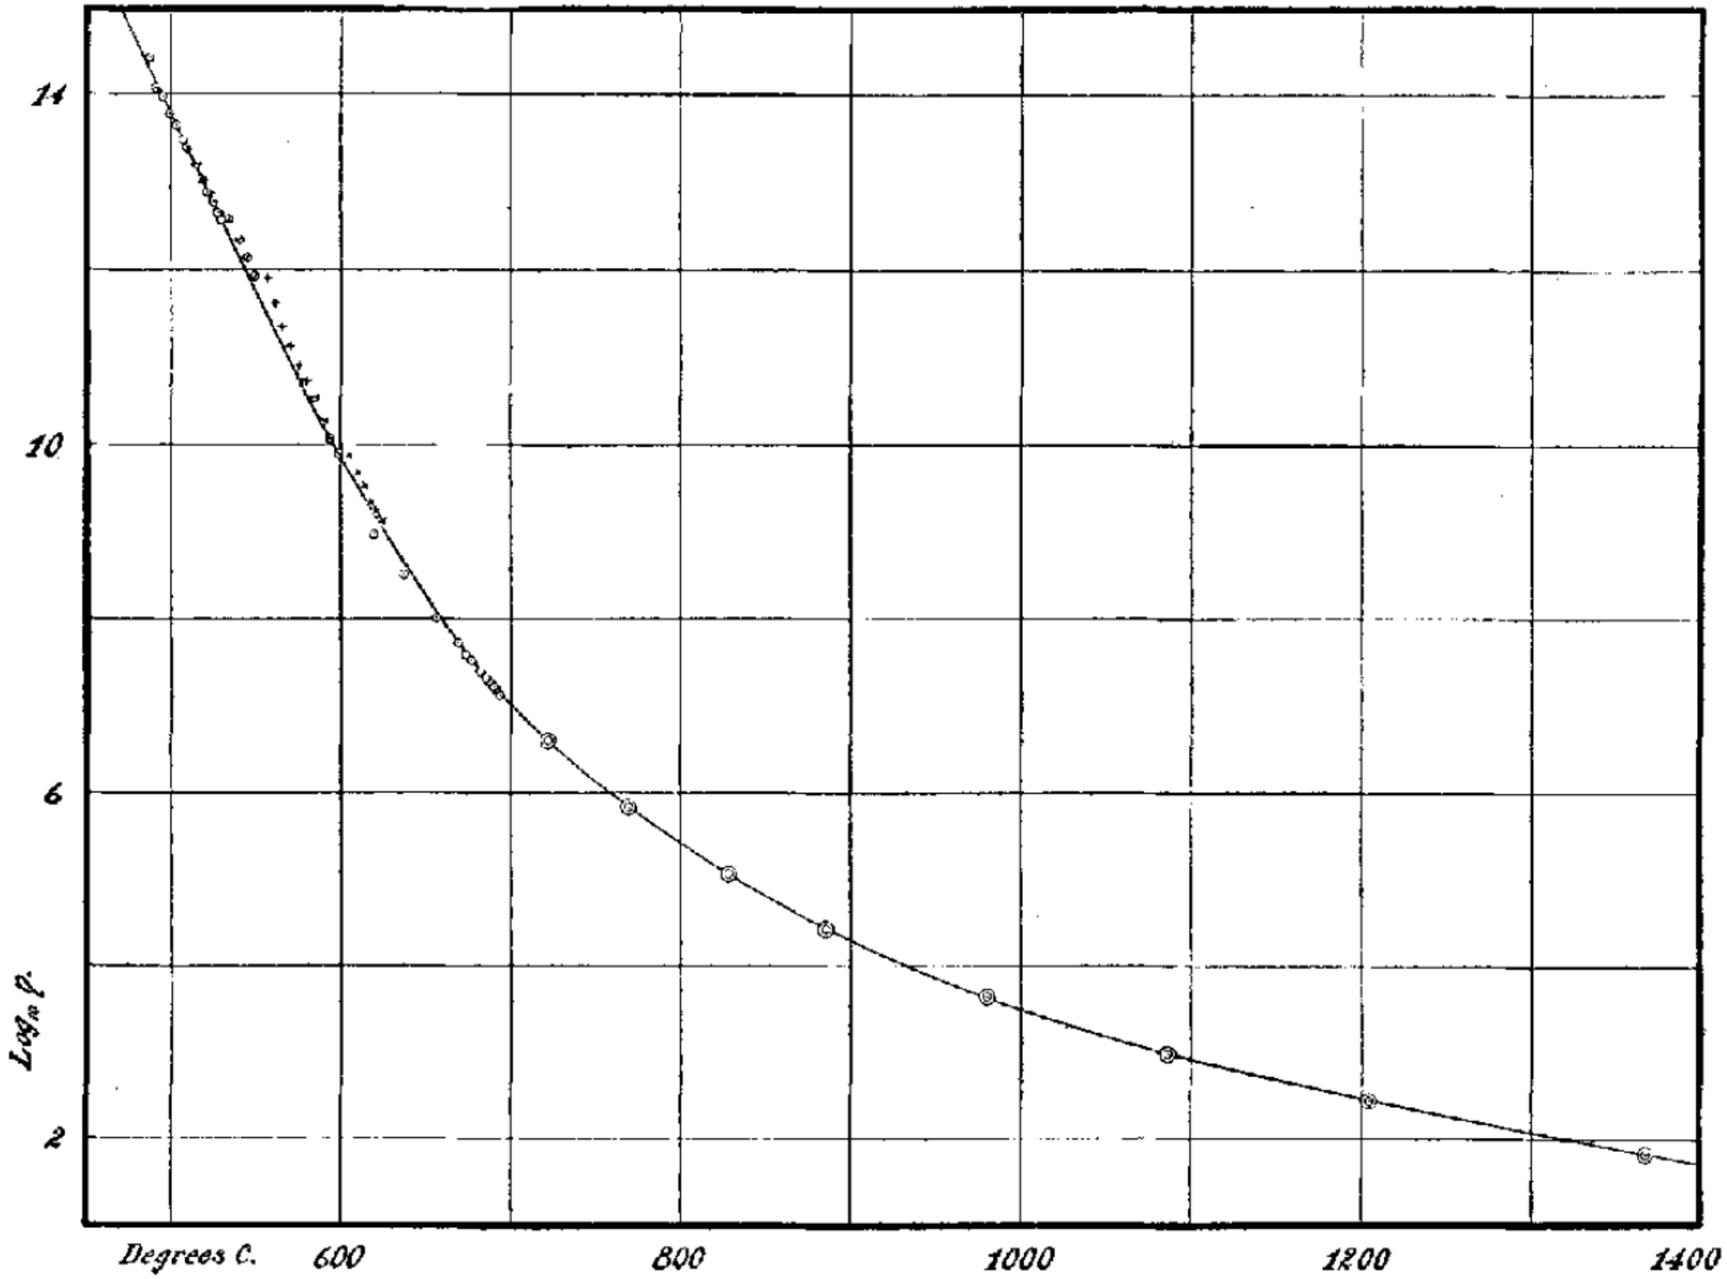


FIG. 5.—Complete viscosity curve for glass I.

H. R. Lillie, J. Amer. Ceram. Soc. **14**, 502 (1931)

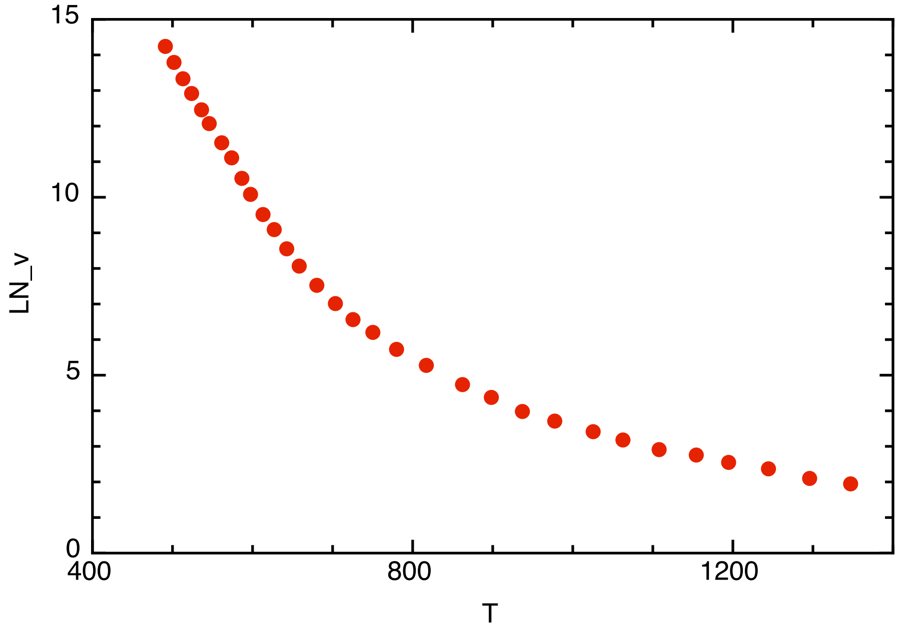


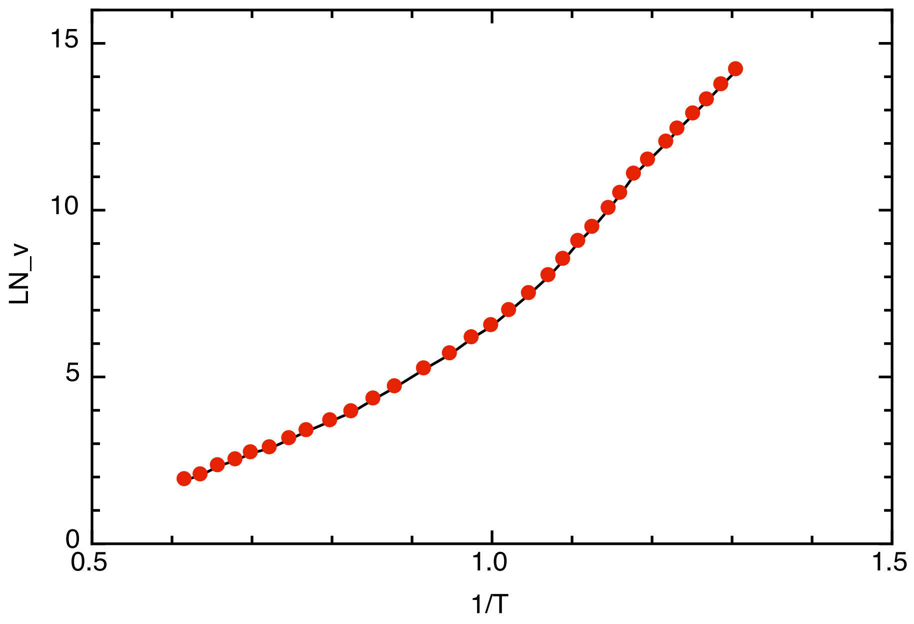


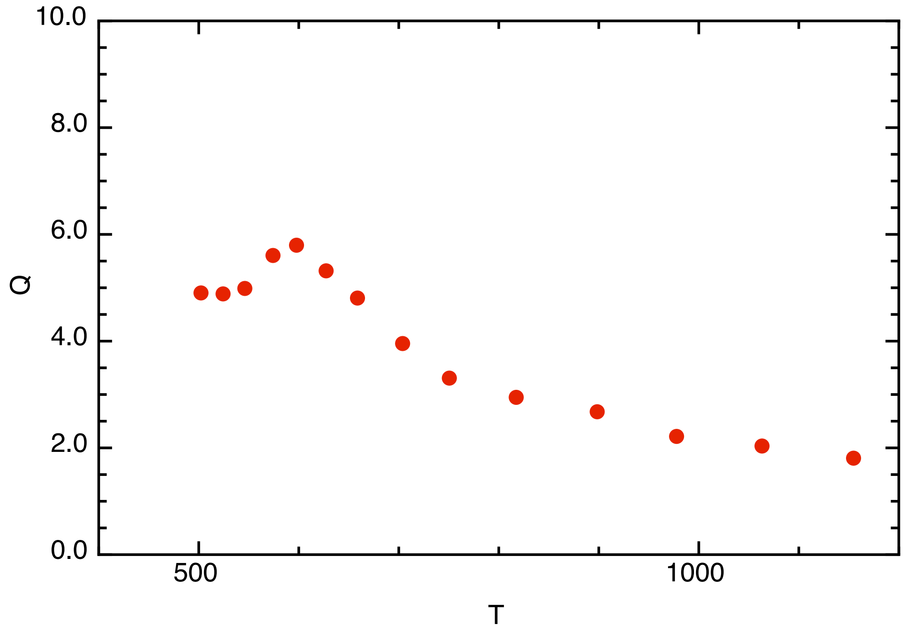


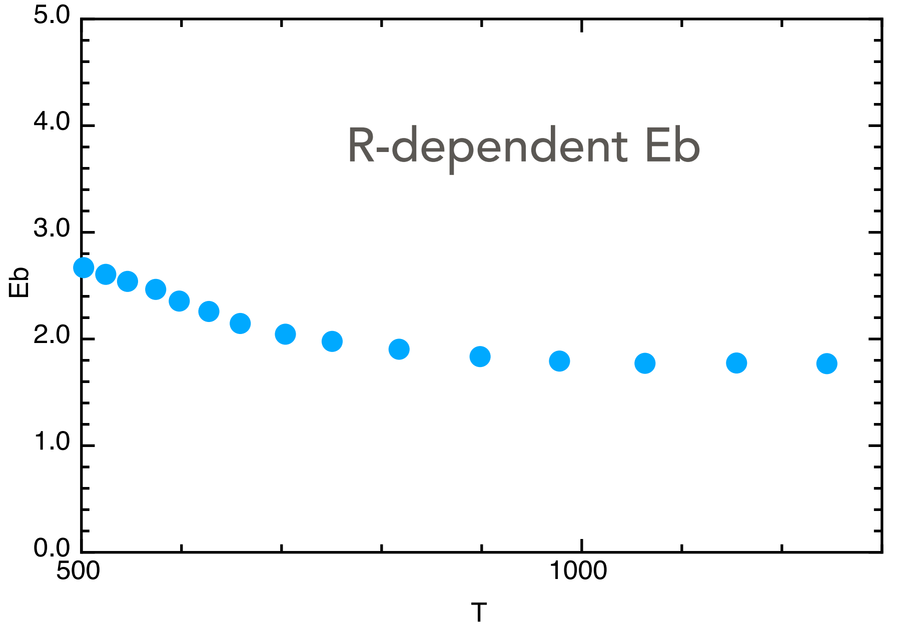

H. R. Lillie, J. Amer. Ceram. Soc. **14**, 502 (1931)

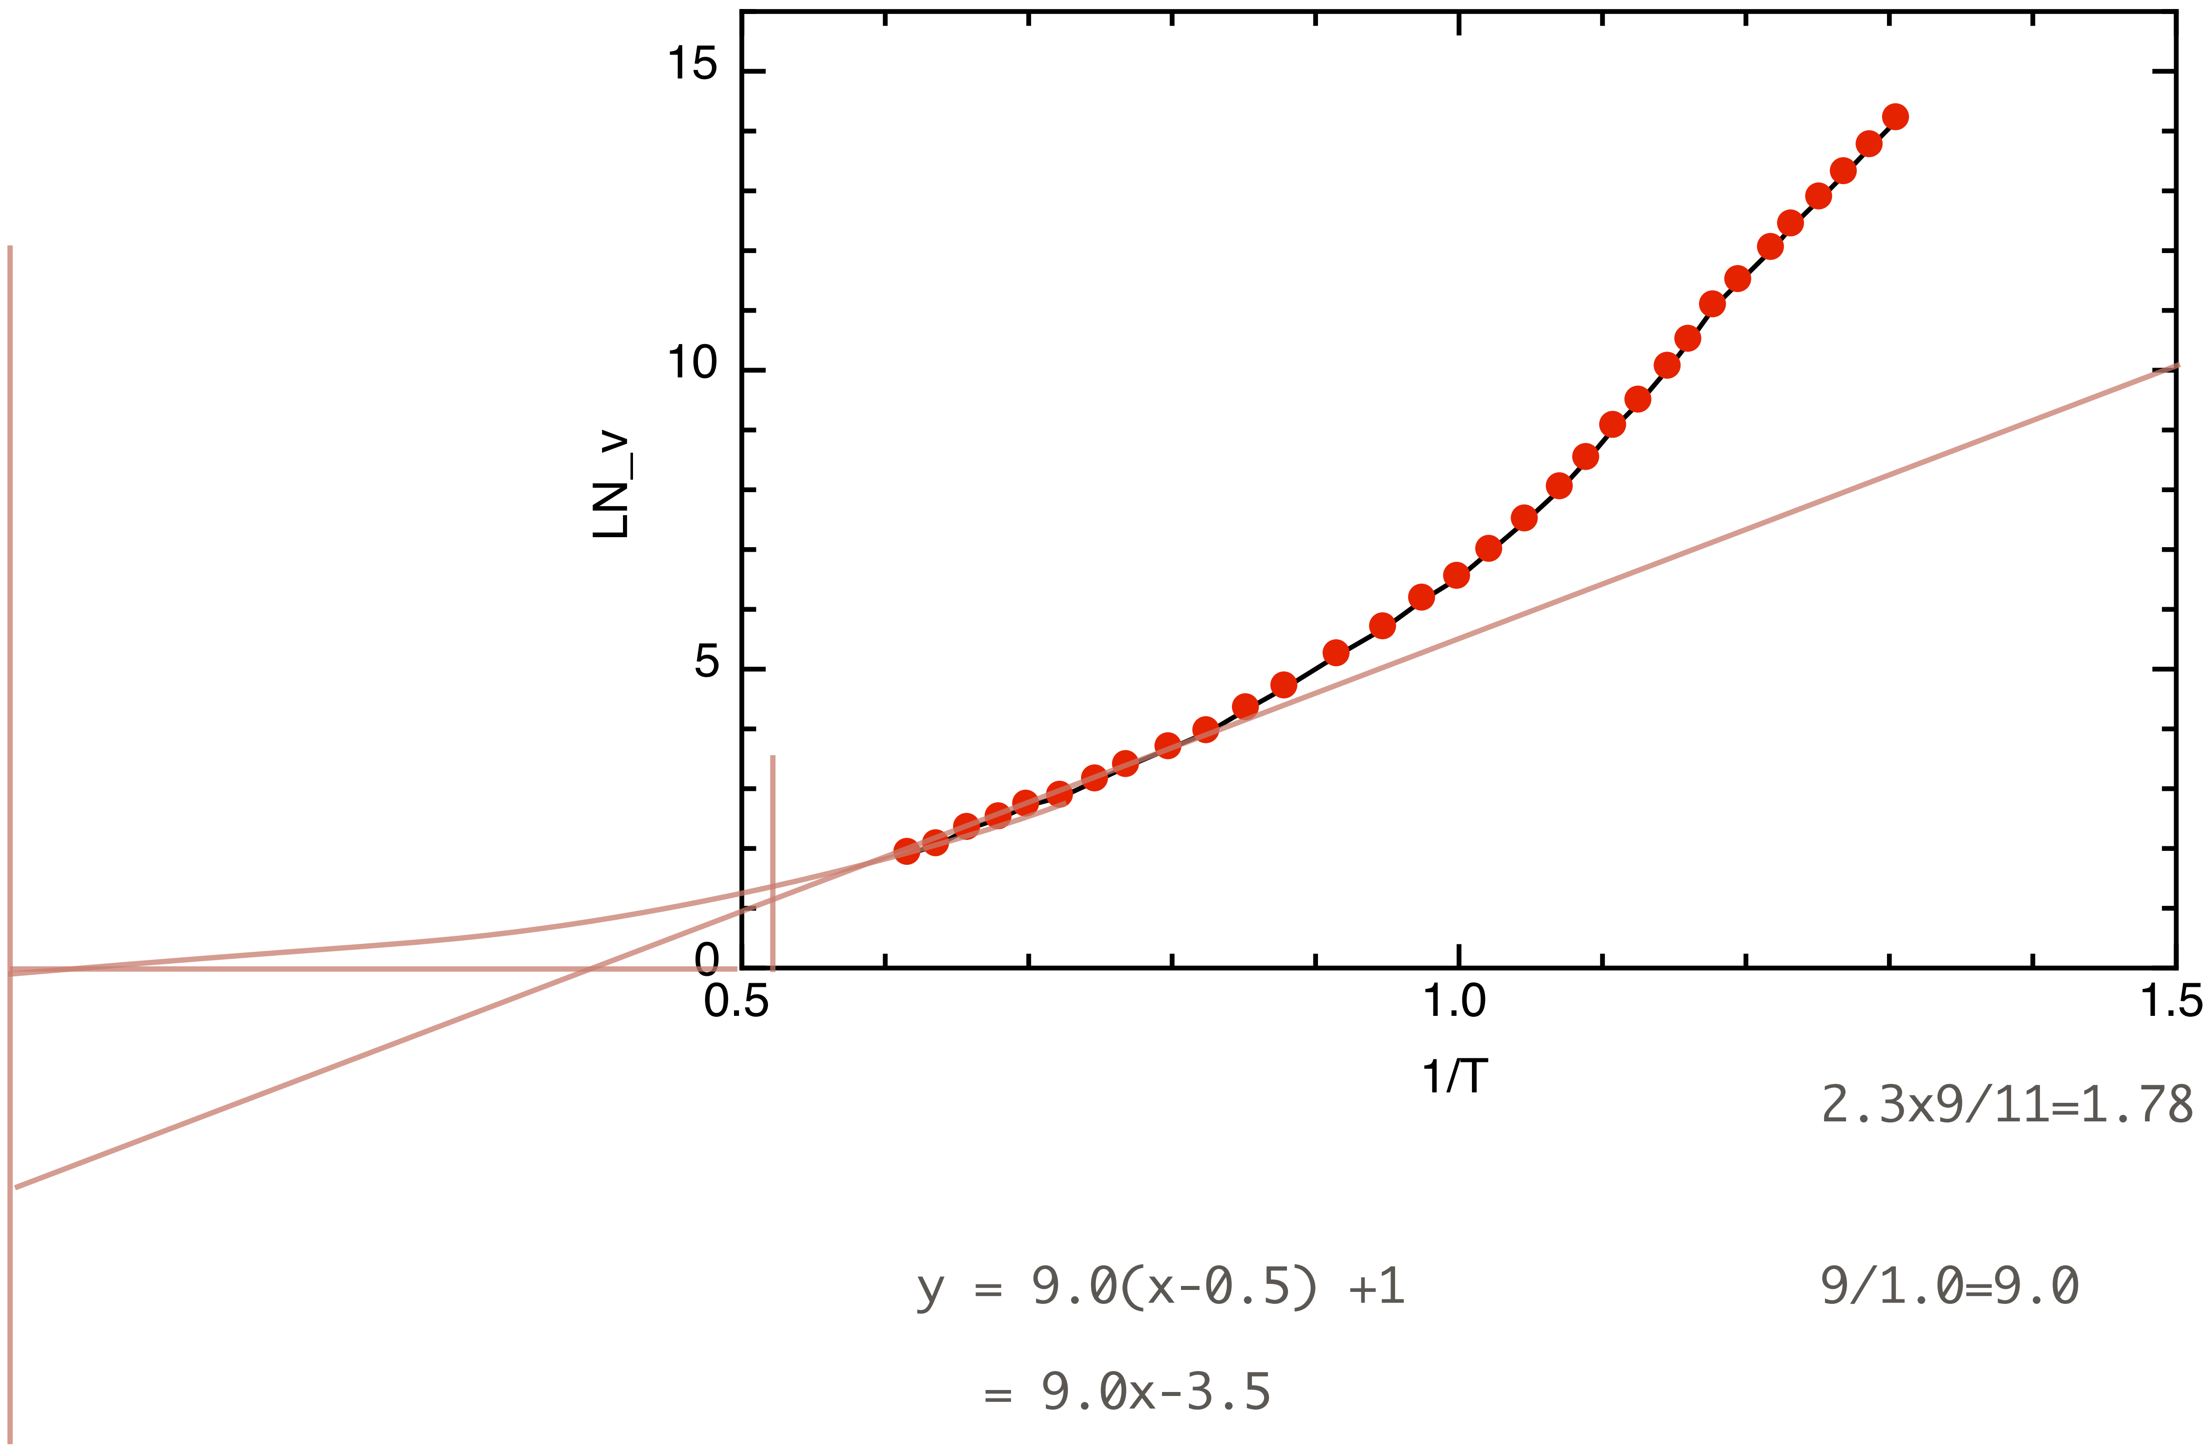


2.3x9/11=1.78

y = 9.0(x-0.5) +1

= 9.0x-3.5

9/1.0=9.0

## Jones data

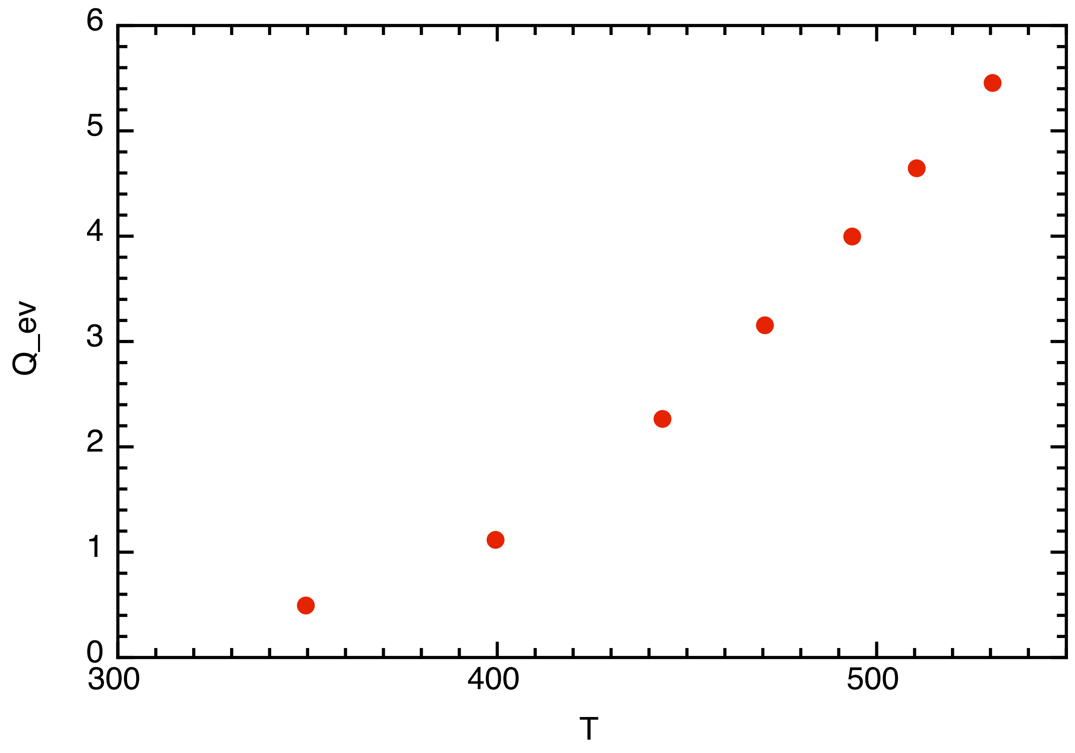


## Lillie data

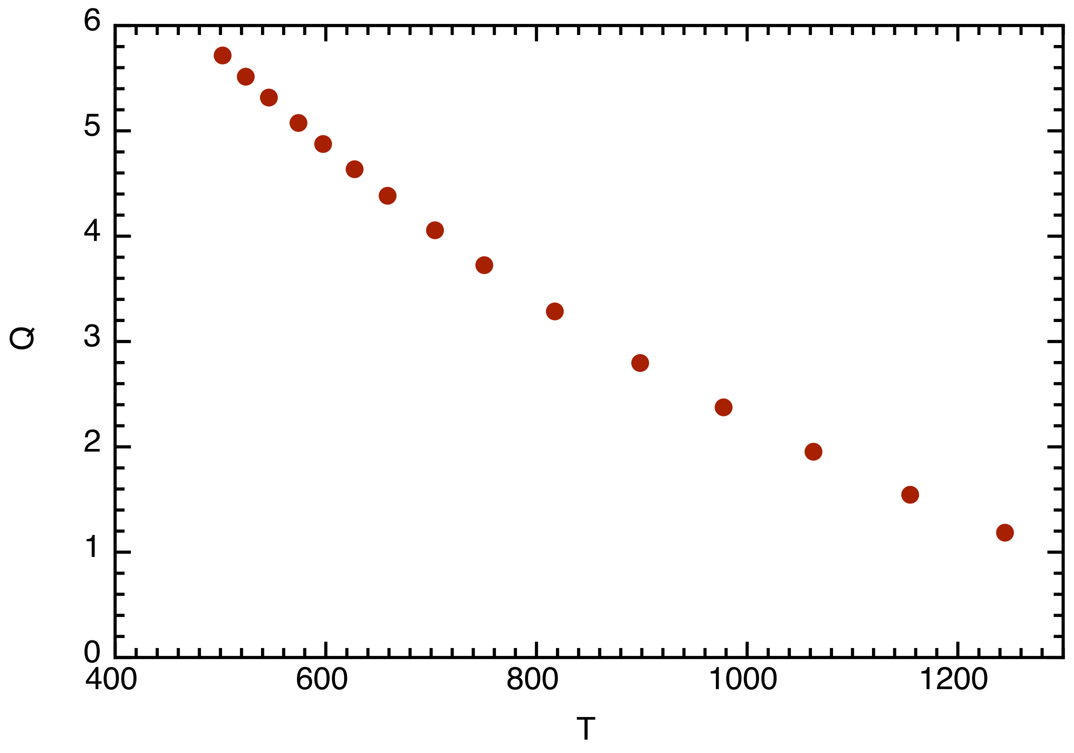

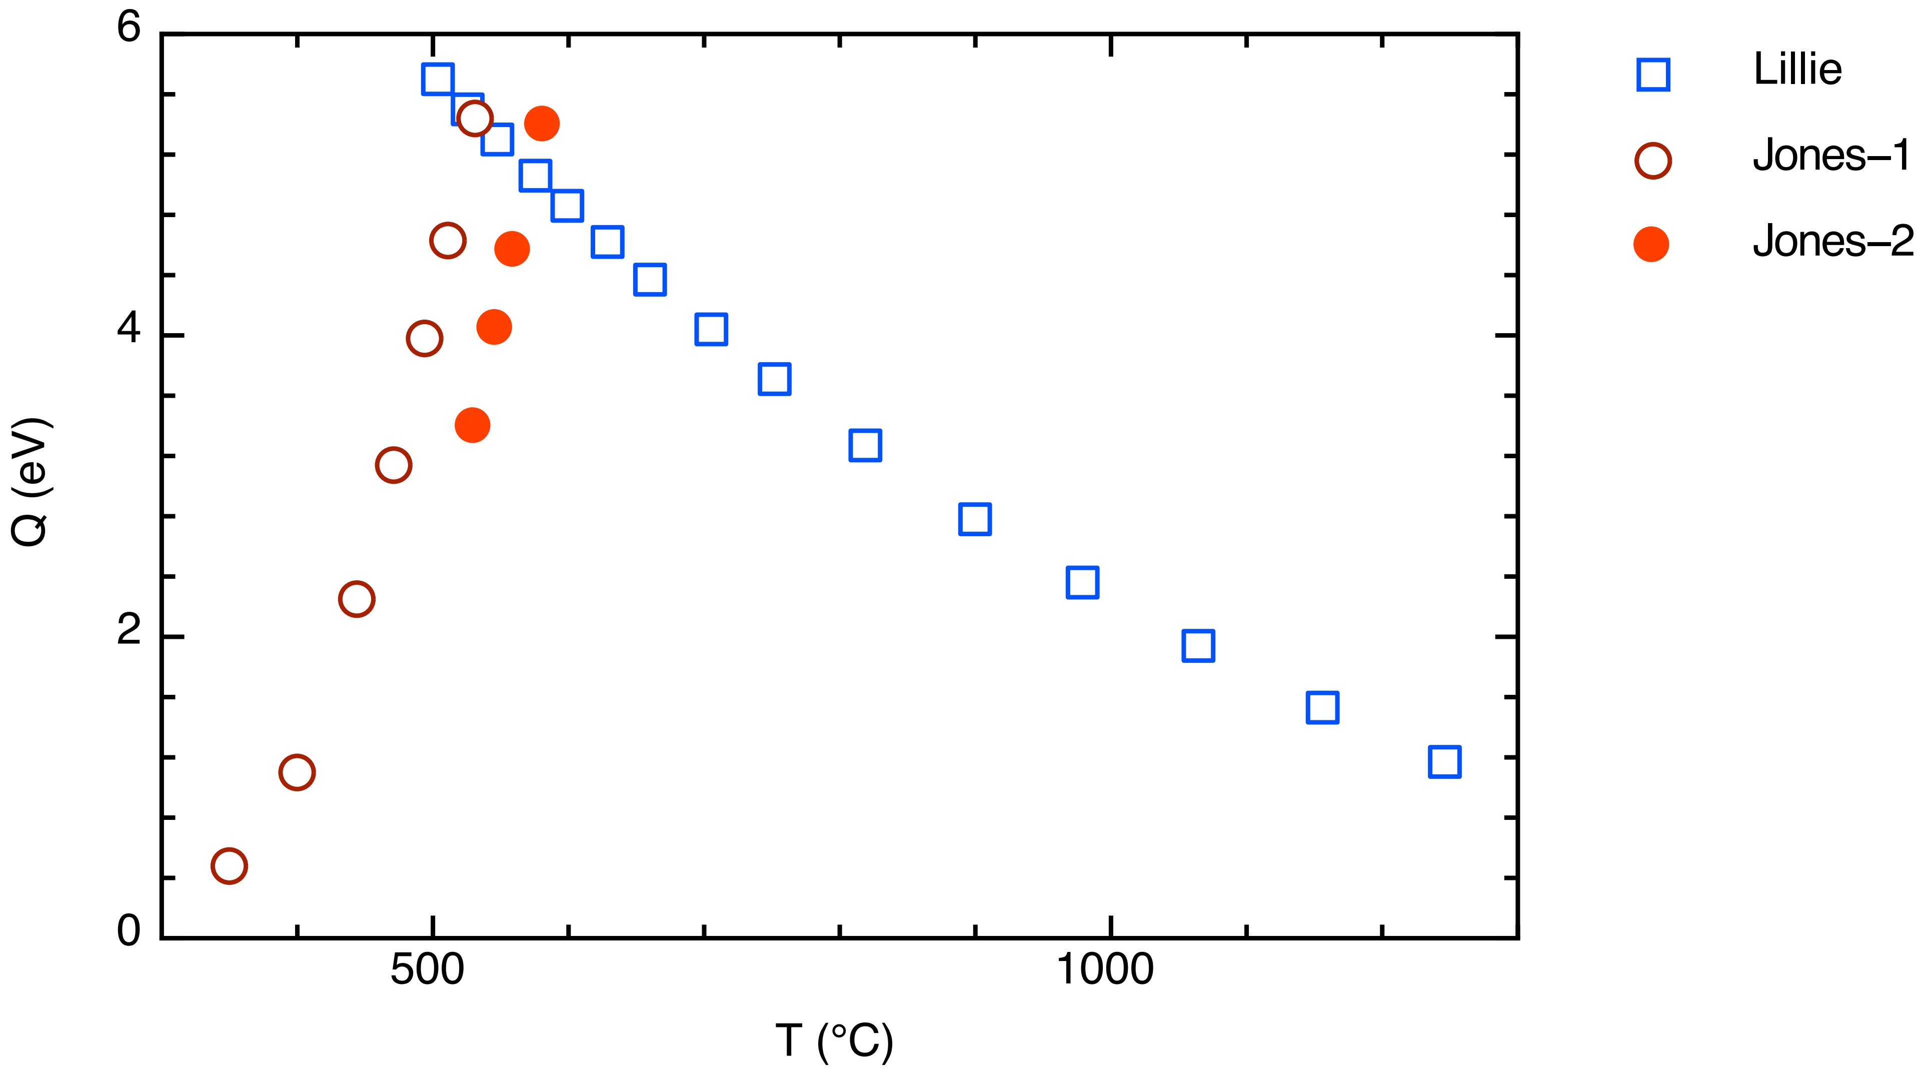

Q (eV)
T (°C)
0
2
4
6
500
1000
Lillie
Jones–1
Jones–2

# Lillie + Jones

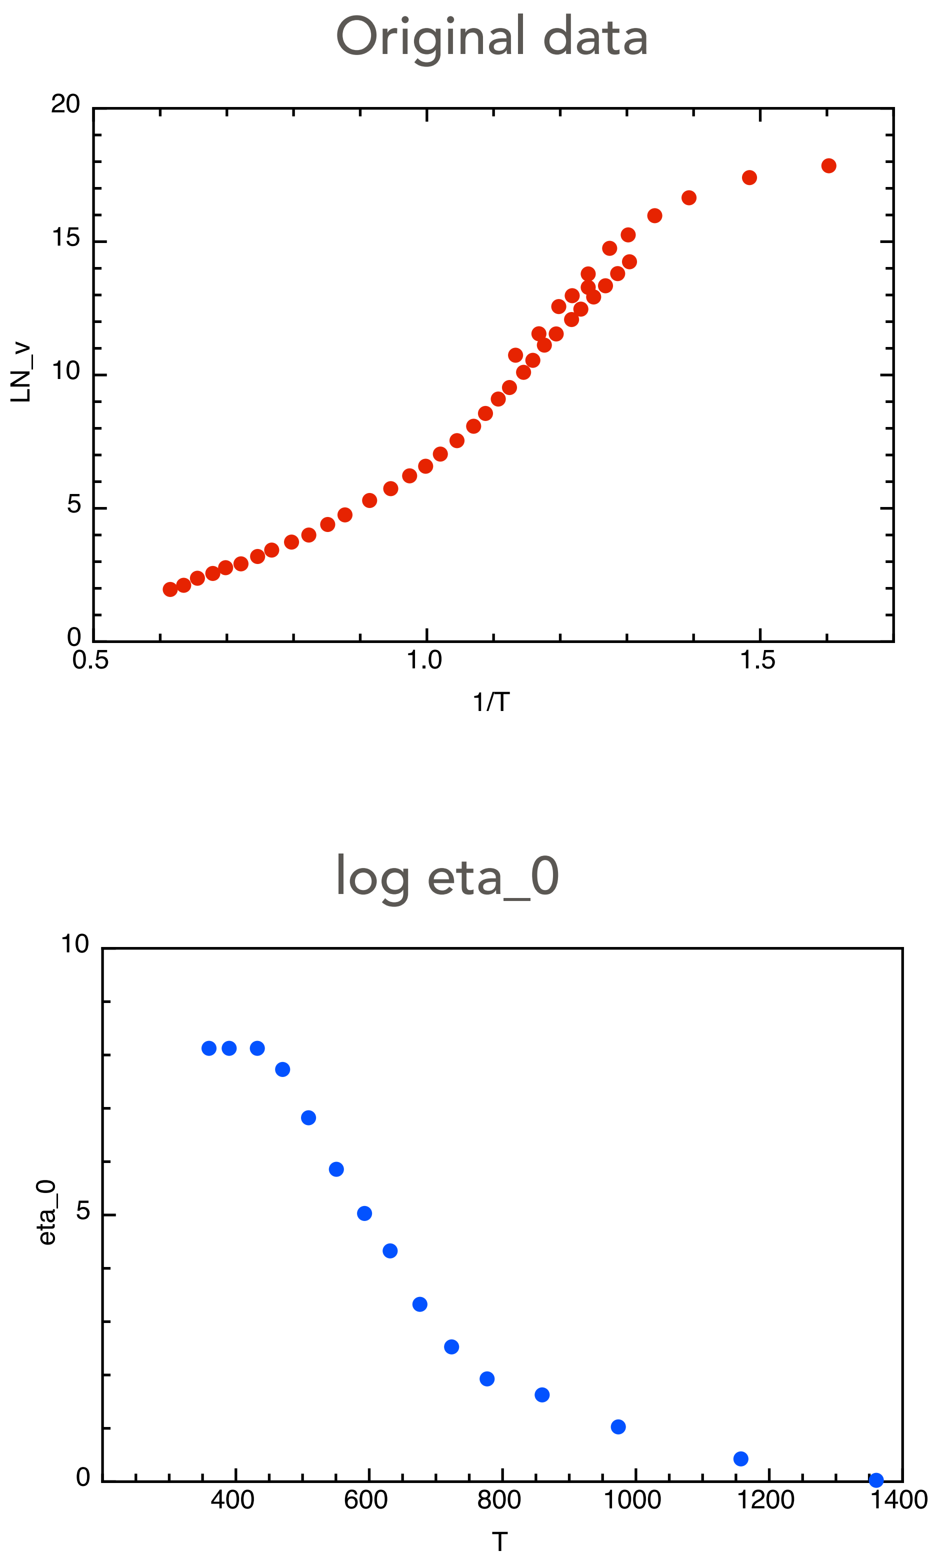

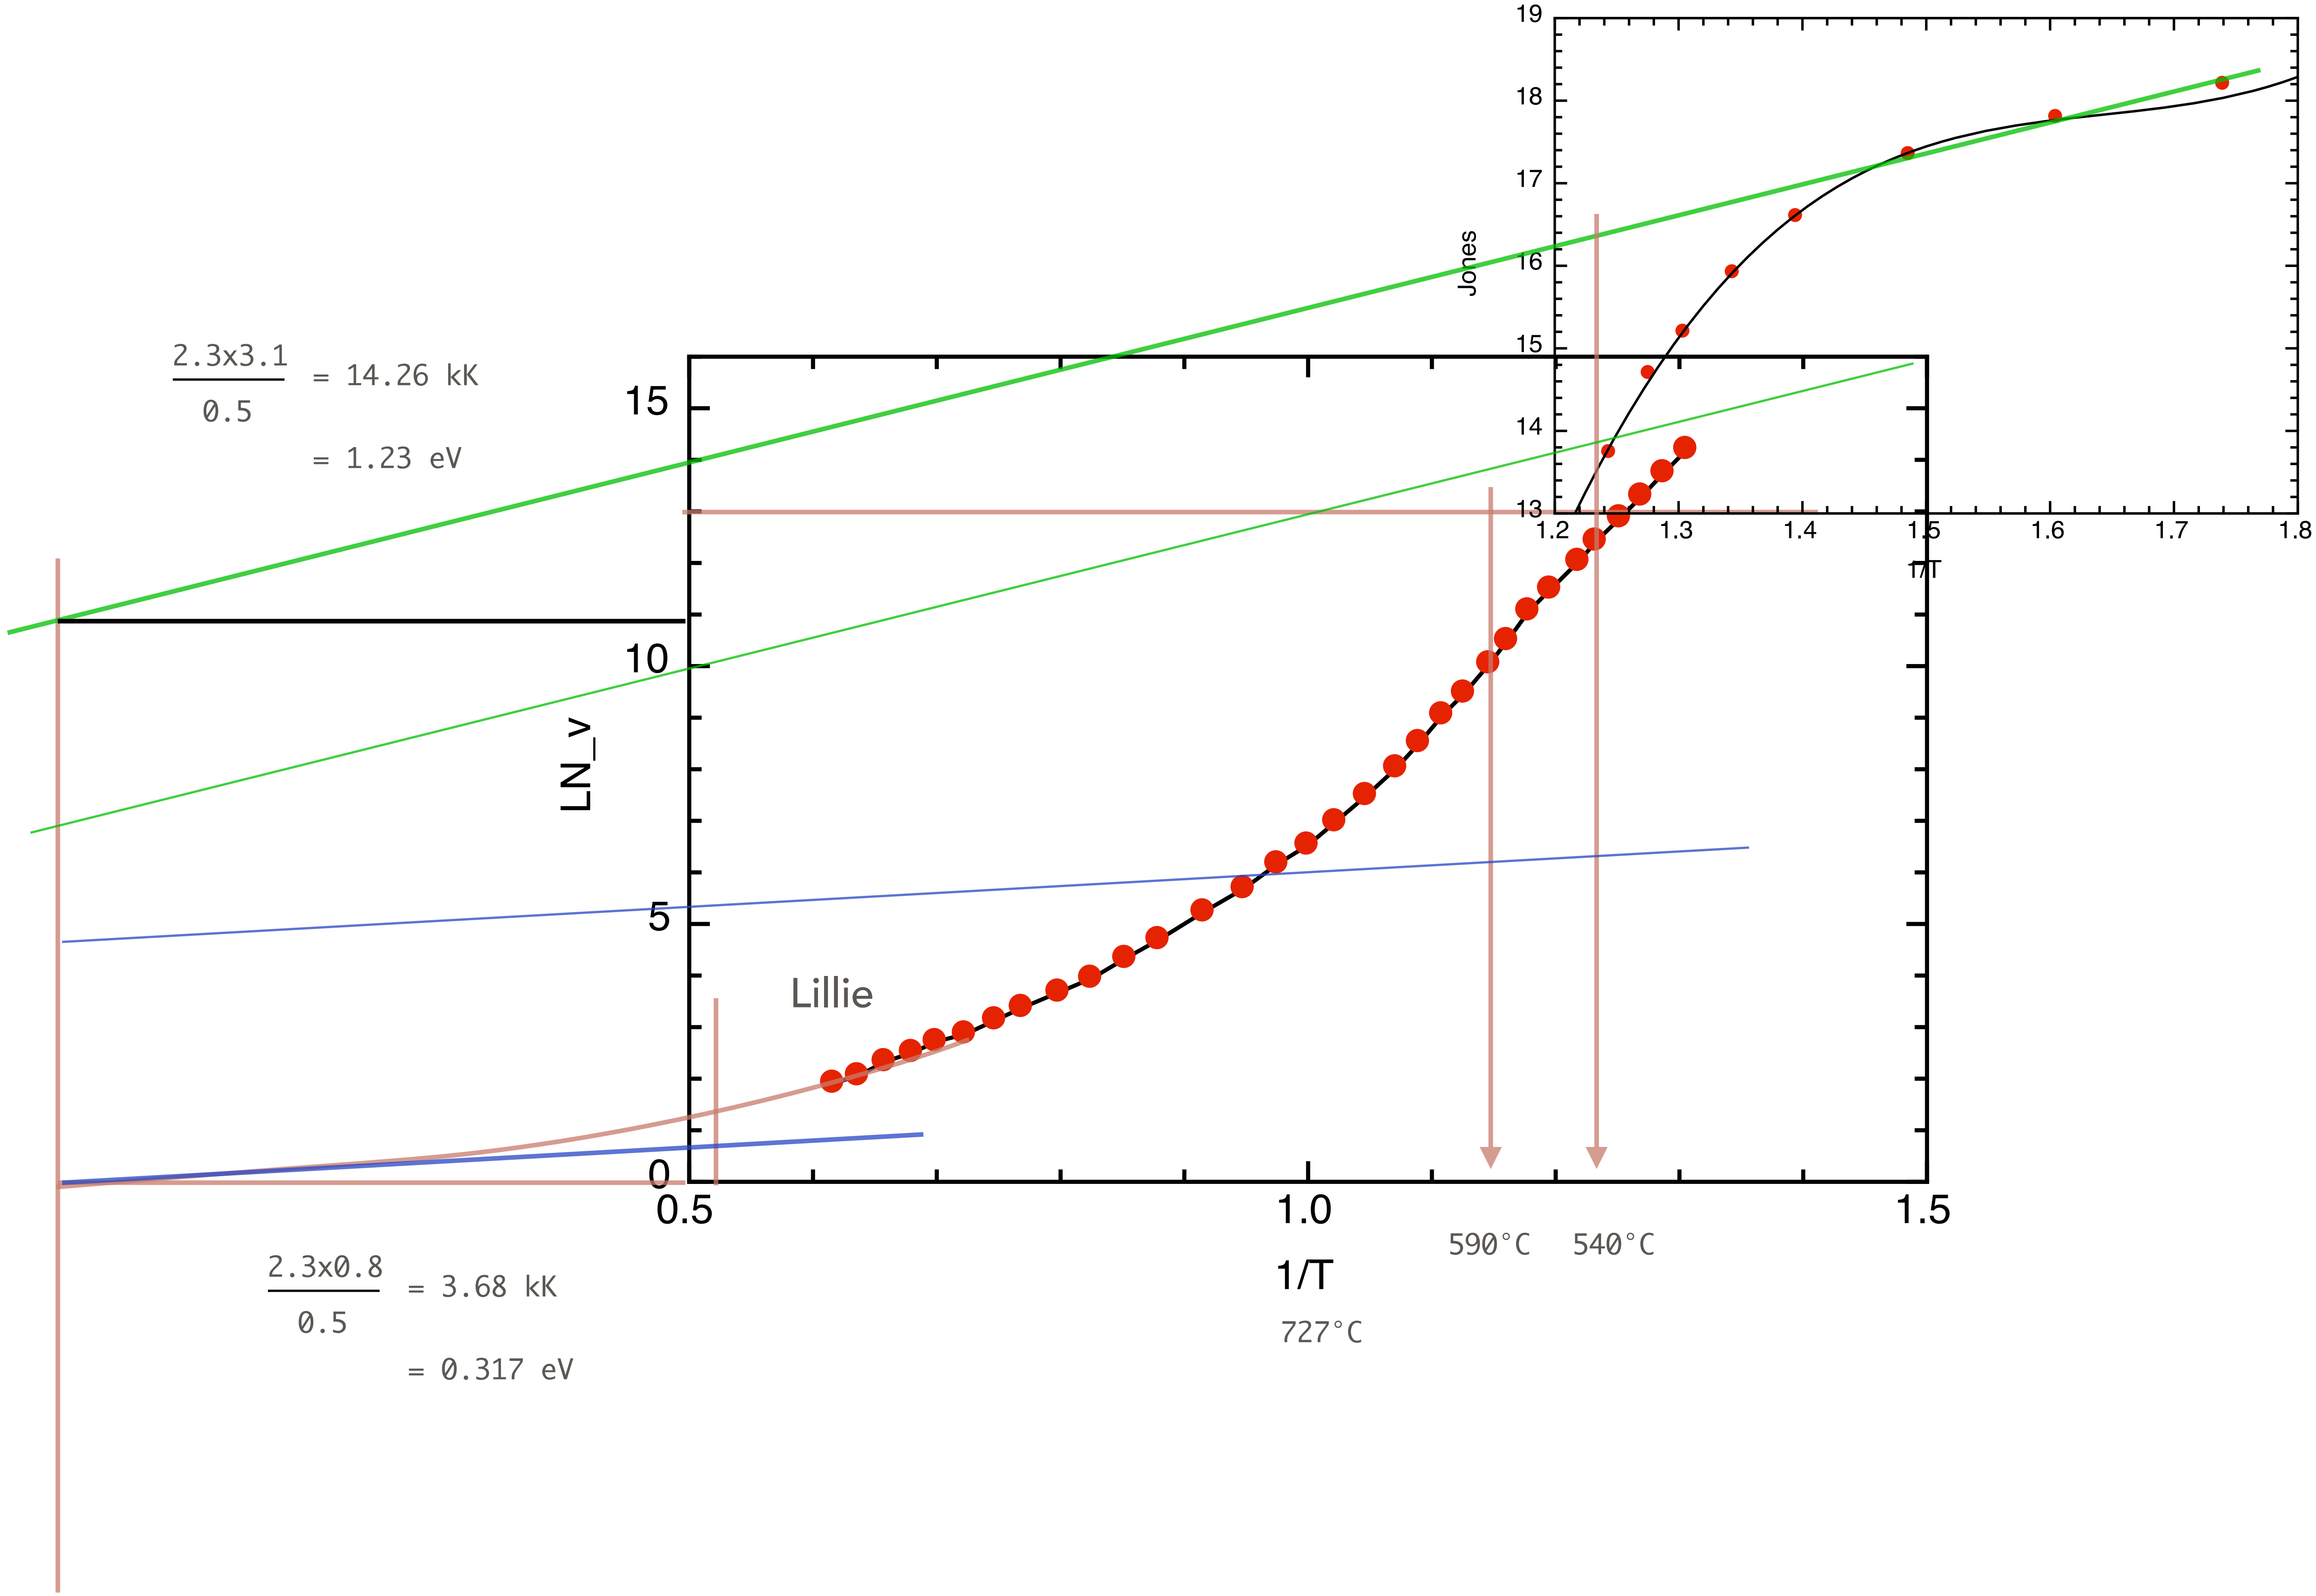

2.3x3.1 / 0.5 = 14.26 kK
= 1.23 eV
LN_v
15
10
5
0
0.5
1.0
1.5
1/T
Lillie
590°C
540°C
727°C
2.3x0.8 / 0.5 = 3.68 kK
= 0.317 eV
Jones
19
18
17
16
15
14
13
1.2
1.3
1.4
1.5
1.6
1.7
1.8
1/T

# Napolitano

A. Napolitano and E. G. Hawkins, J. Res. Natl. Bur. Stand. **68**A, 439 (1964)

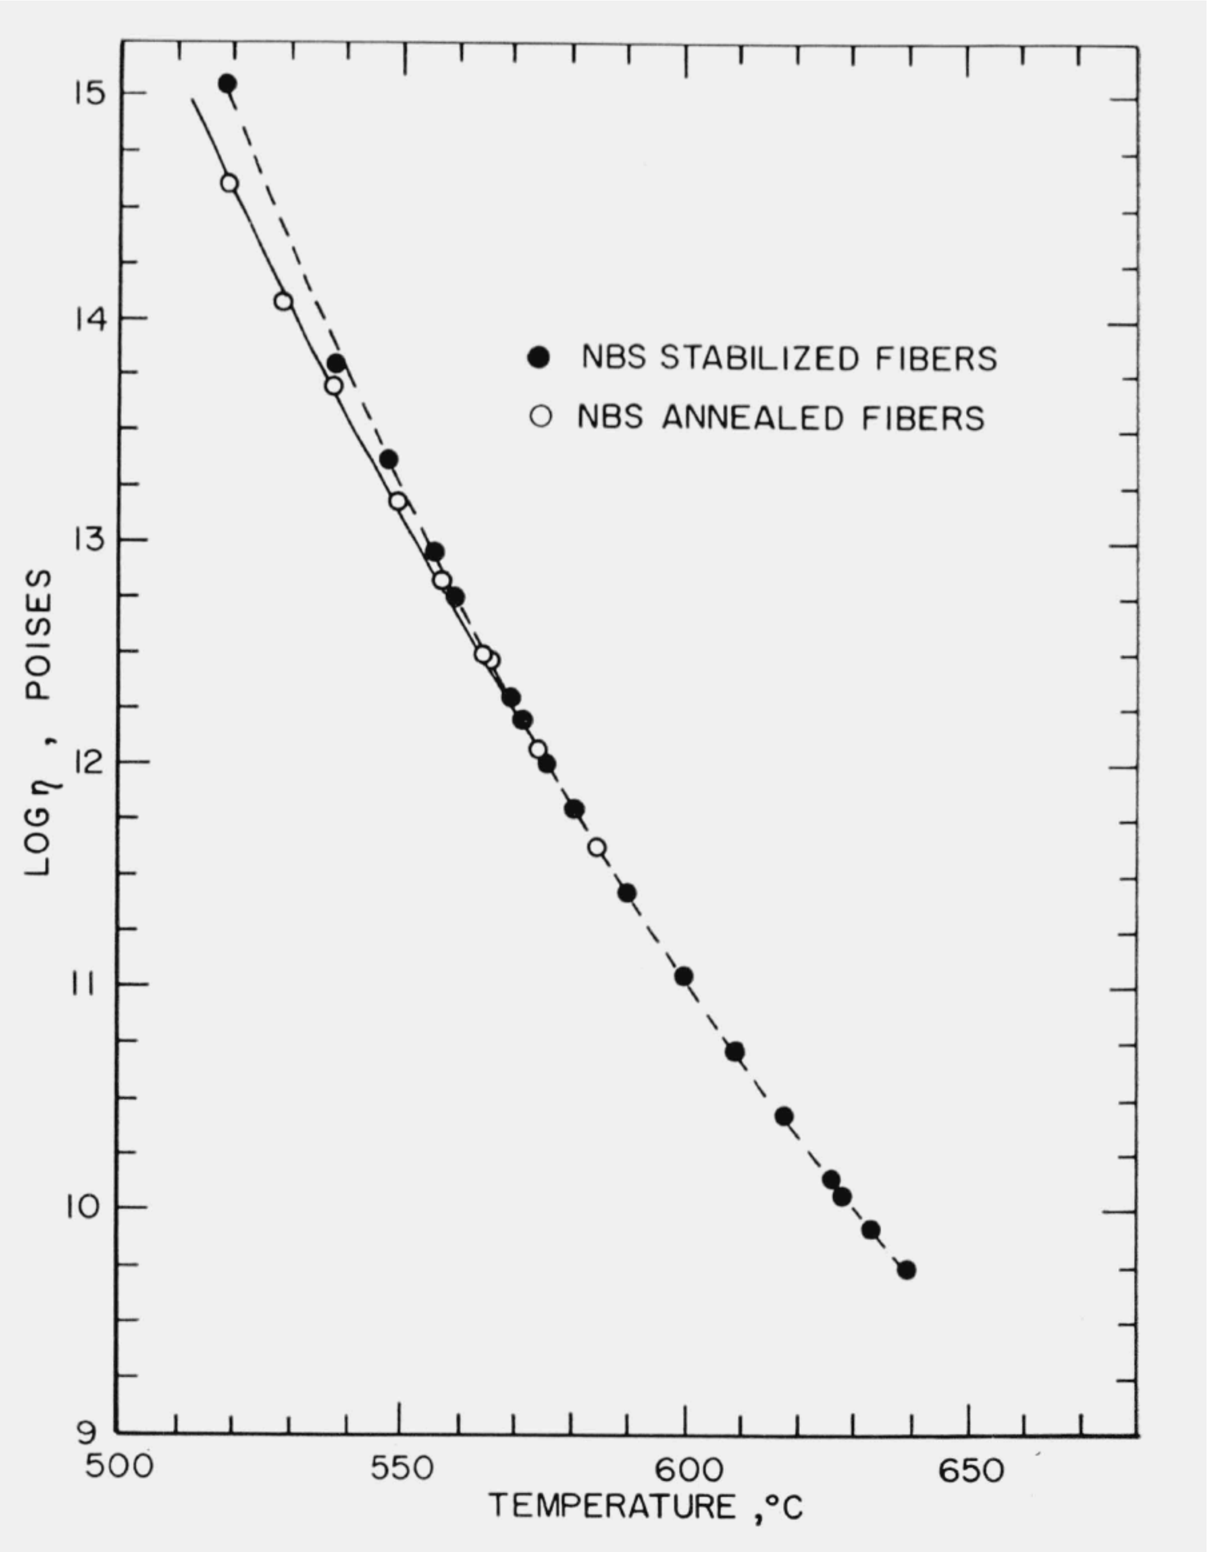

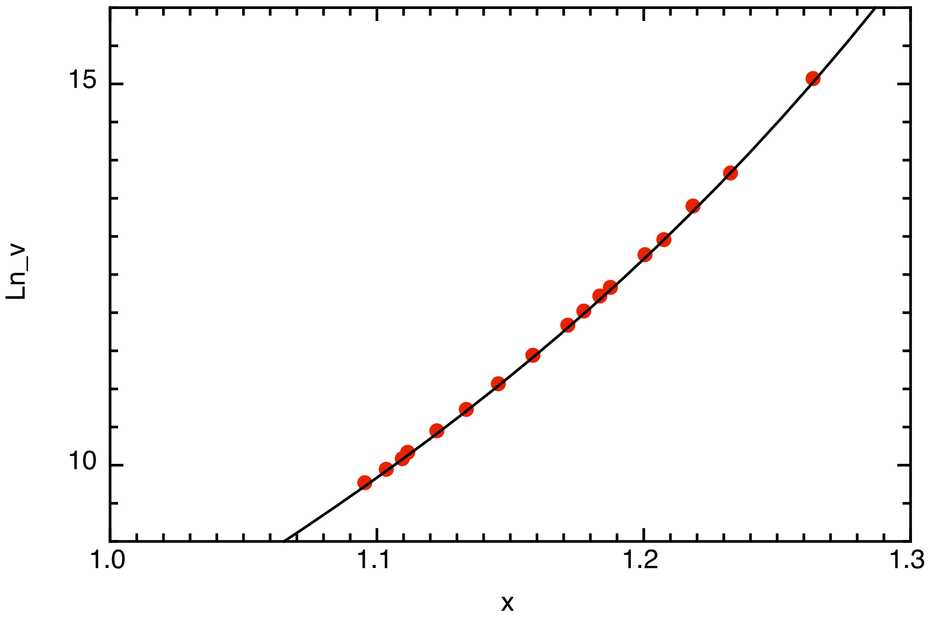


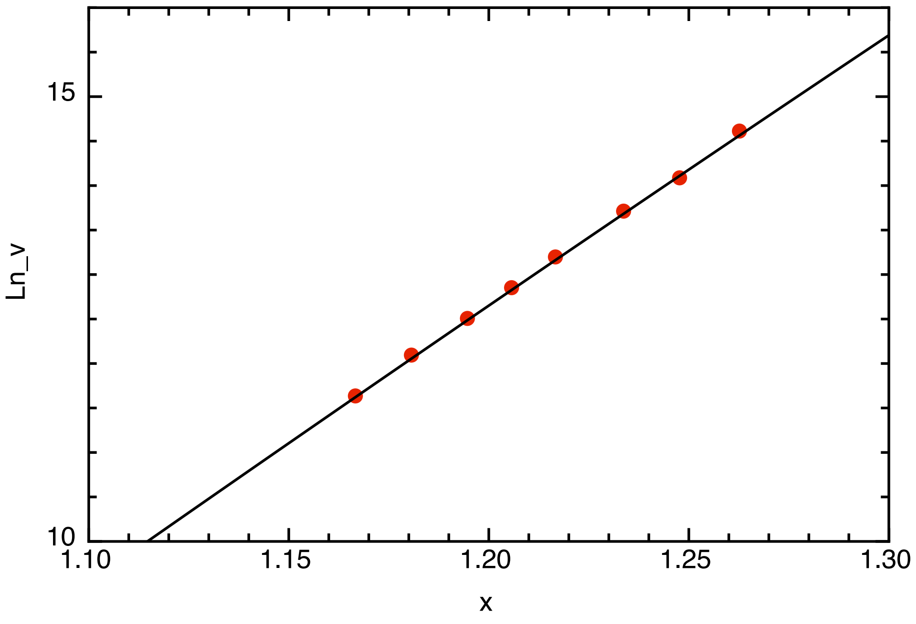


```
Iterations:   1
Seconds   :   0.00012
------------------------------------------
Chi squared          =      0.0047398

Parameters:                           Standard deviations:
deg     =          3.0000
const   =        -74.4785     Δconst =       74.6595
a1      =        212.7652     Δa1    =      190.2047
a2      =       -200.5122     Δa2    =      161.3576
a3      =         69.7915     Δa3    =       45.5822

Coefficient of Determination :            0.9999
Mean value of y-values y[i]  :            11.7525
Sum of squares of y[i]-yMean :            36.9251
Sum of squares of residuals  :            0.0047398
```

```
Iterations:   1
Seconds   :   2.2e-5
------------------------------------------
Chi squared          =      0.0031693

Parameters:                           Standard deviations:
deg     =          2.0000
const   =        -29.4830     Δconst =      15.1411
a1      =         39.4693     Δa1    =      24.9304
a2      =         -3.6315     Δa2    =      10.2569

Coefficient of Determination :            0.9996
Mean value of y-values y[i]  :            13.0733
Sum of squares of y[i]-yMean :            7.2232
Sum of squares of residuals  :            0.0031693
```

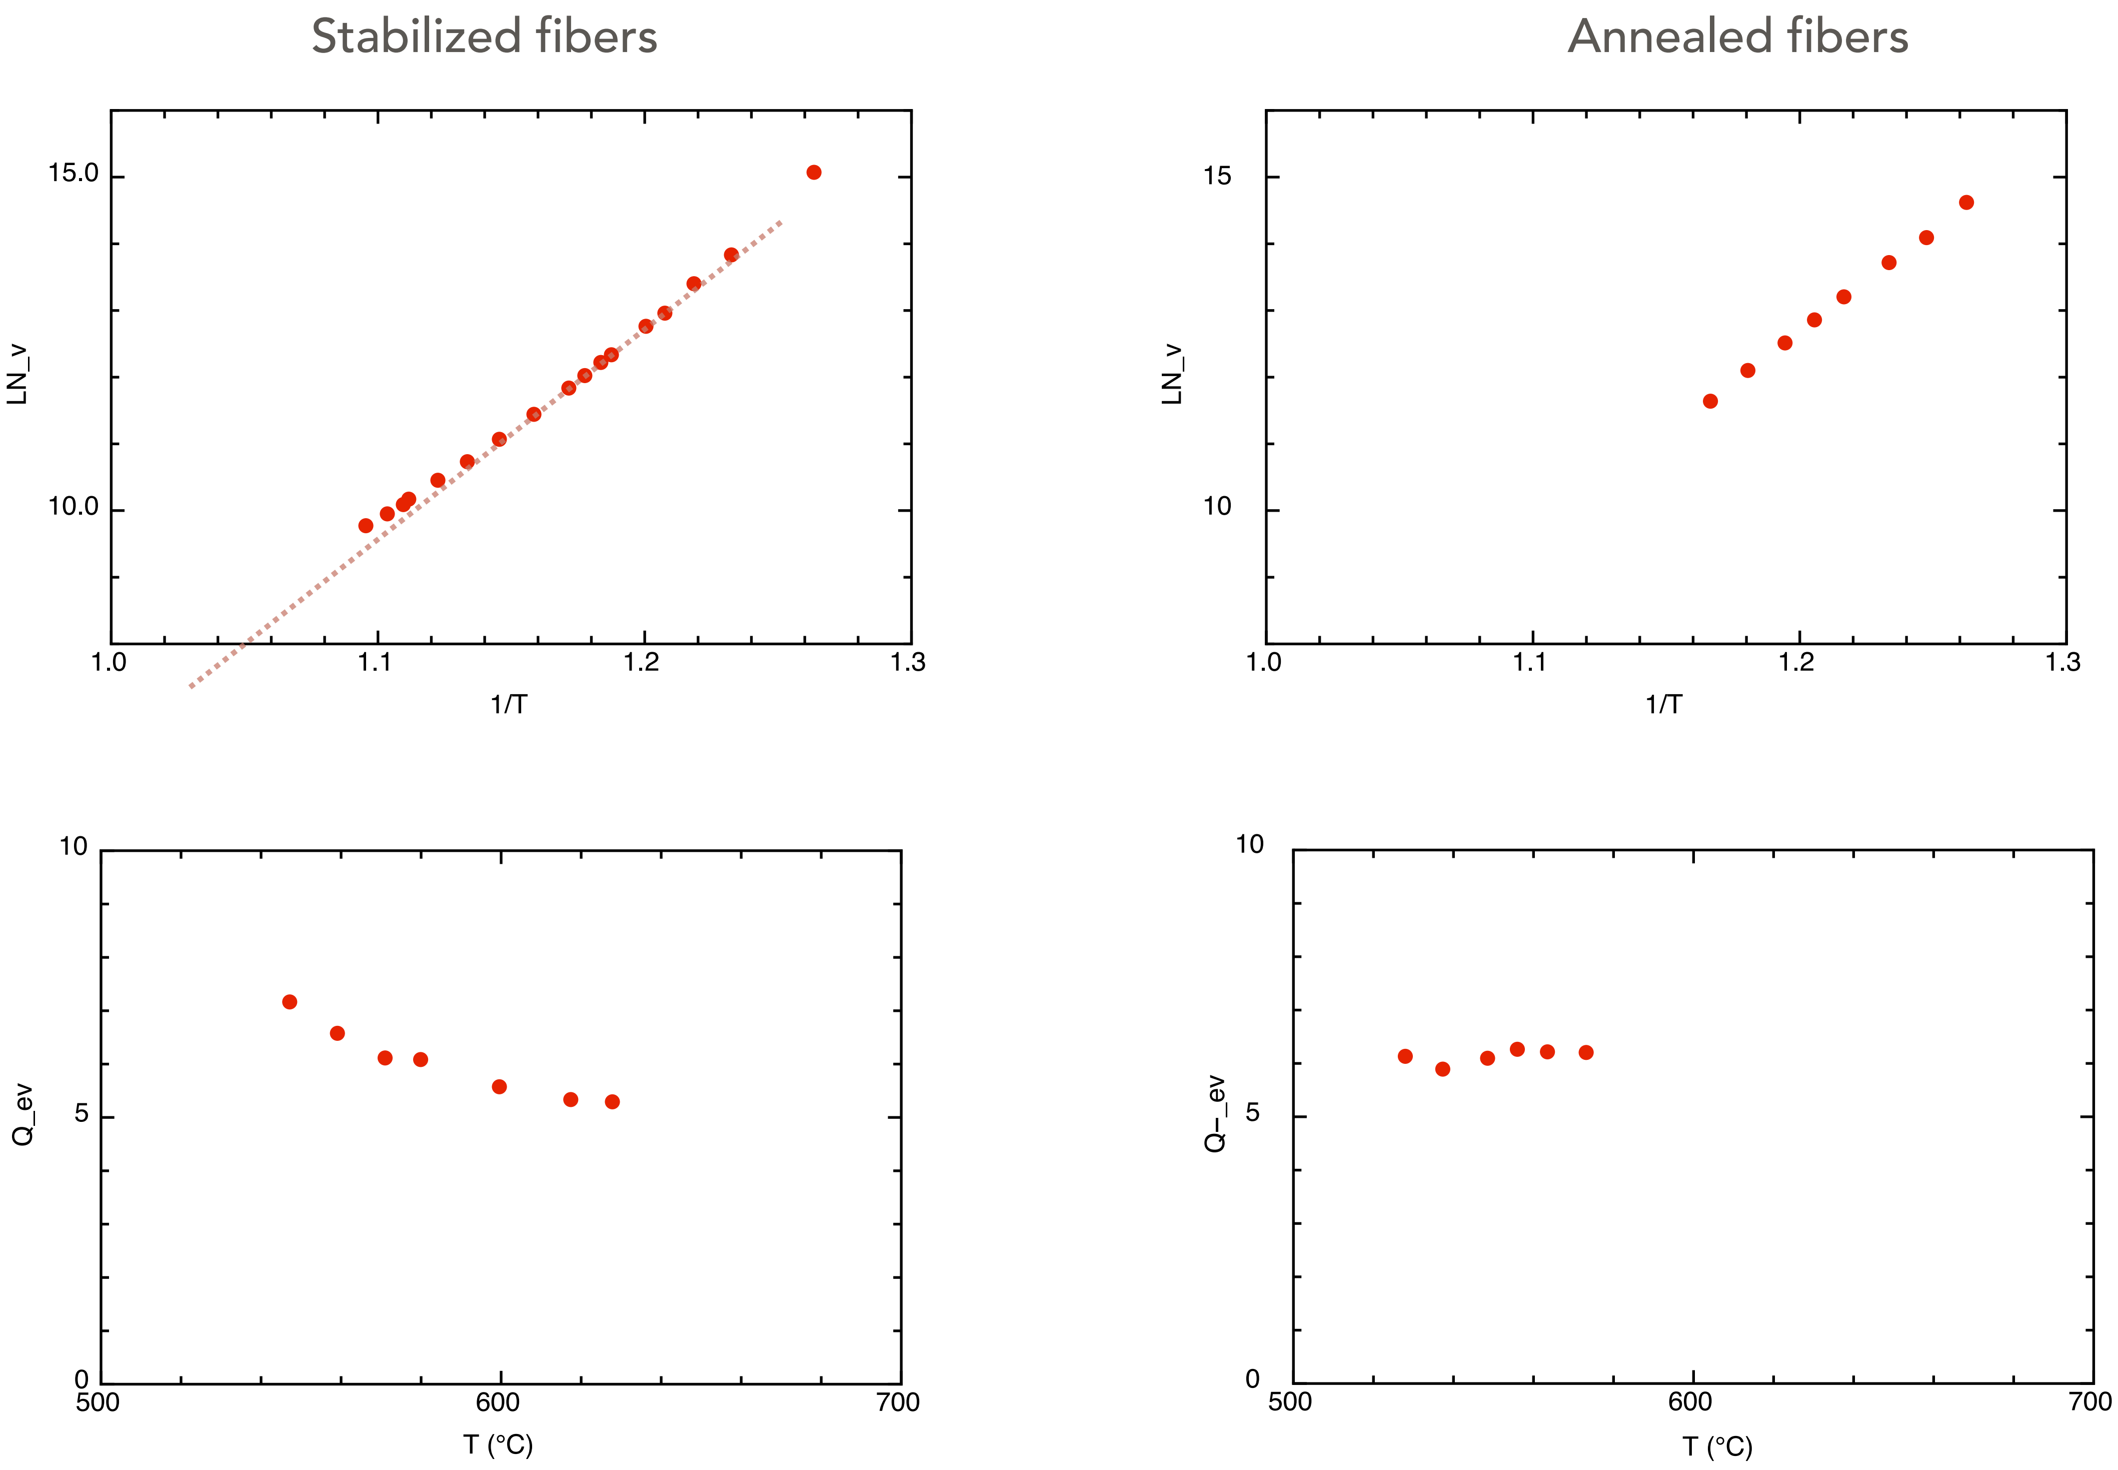
Stabilized fibers
Annealed fibers
LN_v
15.0
10.0
1/T
1.0
1.1
1.2
1.3
LN_v
15
10
1/T
1.0
1.1
1.2
1.3
Q_ev
10
5
0
T (°C)
500
600
700
Q–_ev
10
5
0
T (°C)
500
600
700

# Mazurin

O. V. Mazurin et al., Sov. J. Glass Phys. Chem., **1**, 494 (1975)

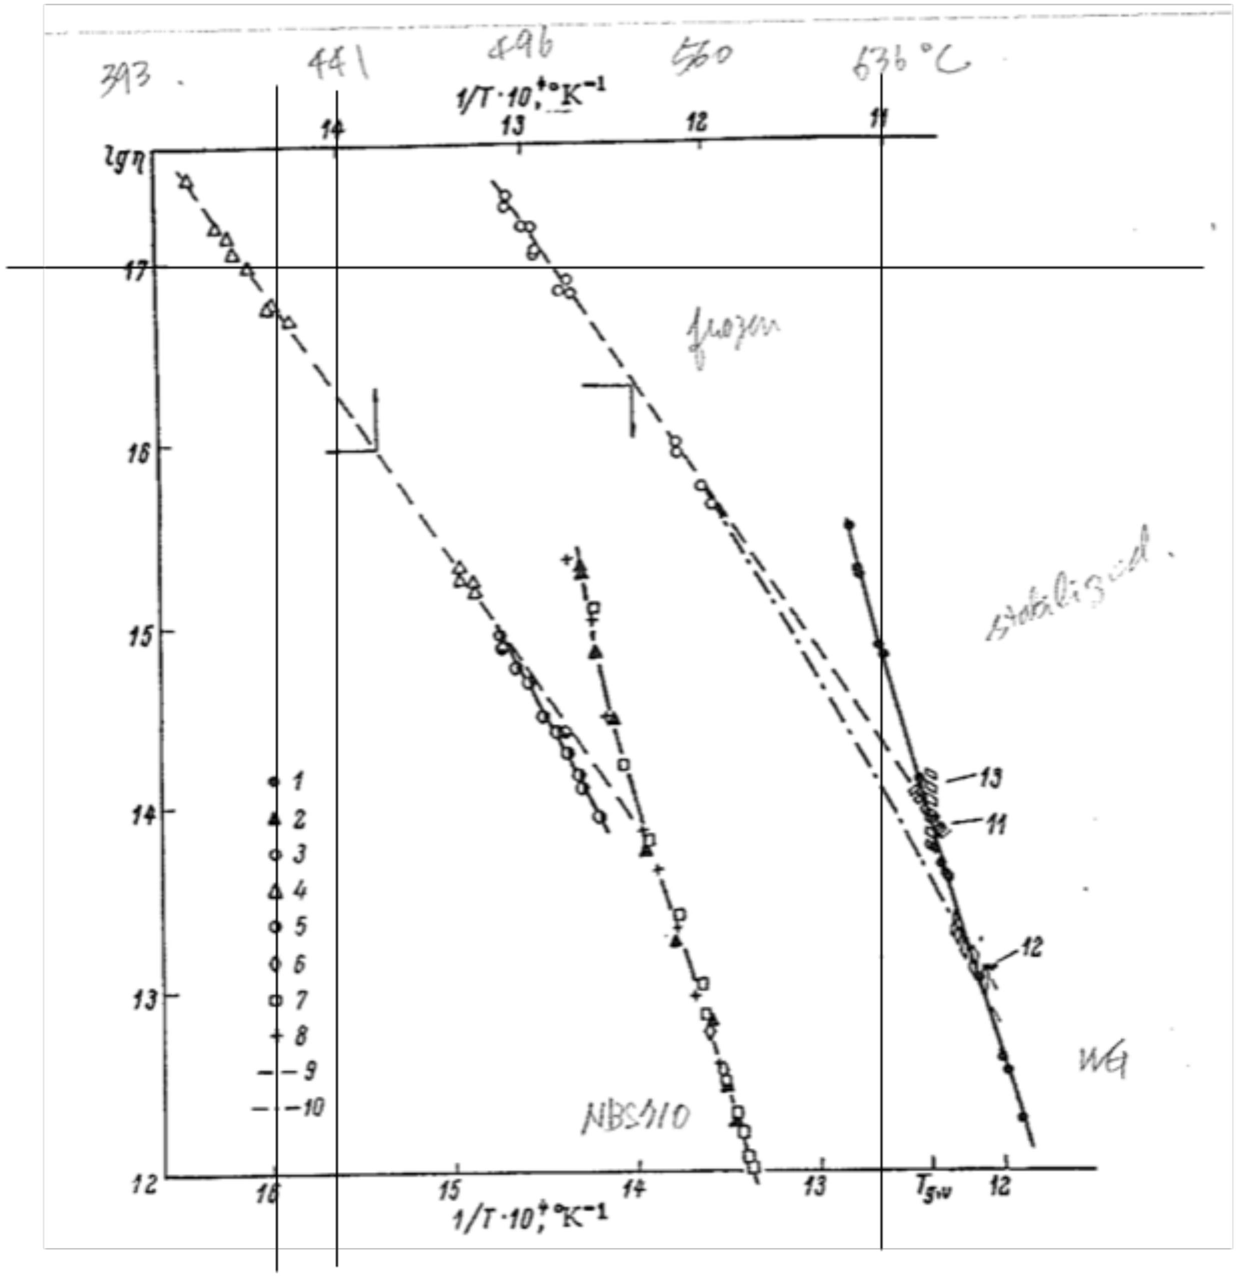

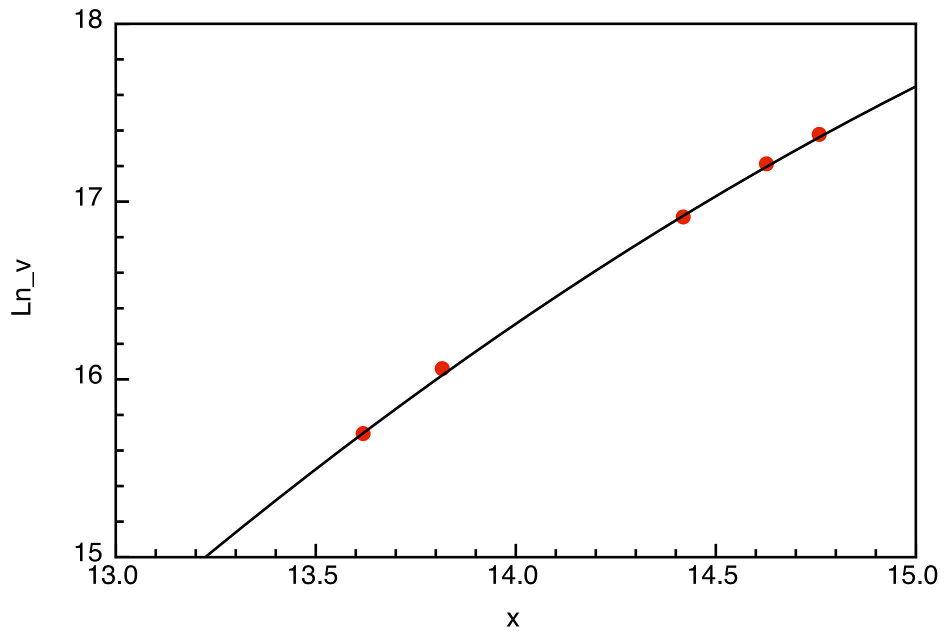


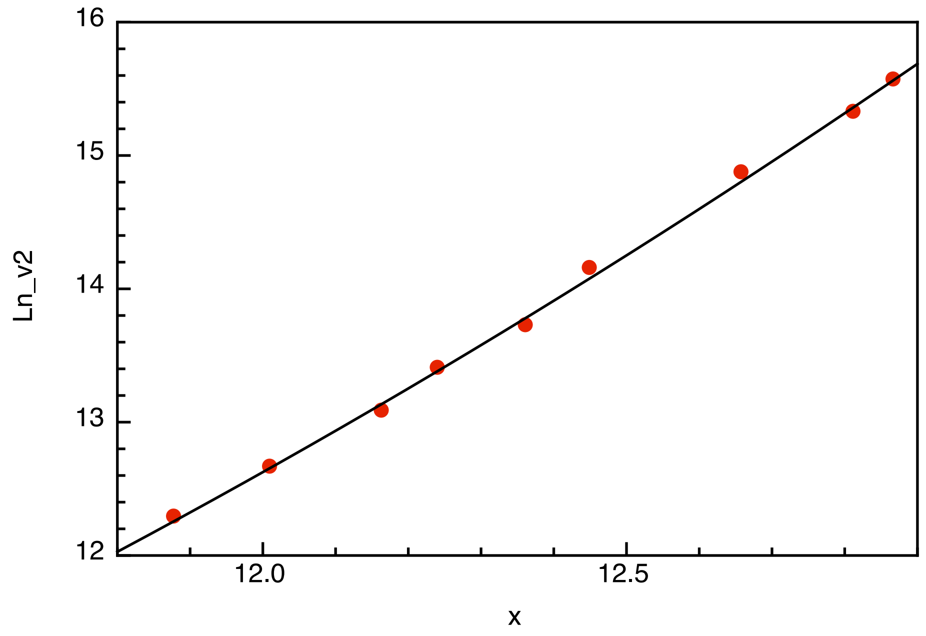


```
Iterations:  1
Seconds    :  0.000114
-------------------------------------------
Chi squared        =      0.0012414

Parameters:                        Standar:
deg    =        2.0000
const  =      -44.3831     Δconst =      21.1511
a1     =        7.1355     Δa1    =       2.9852
a2     =       -0.2000     Δa2    =       0.1052
```

```
Iterations:  1
Seconds    :  2.5e-5
-------------------------------------------
Chi squared        =      0.018893

Parameters:                        Standard:
deg    =        2.0000
const  =       30.3441     Δconst =      30.7504
a1     =       -6.0151     Δa1    =       4.9644
a2     =        0.3782     Δa2    =       0.2003
```

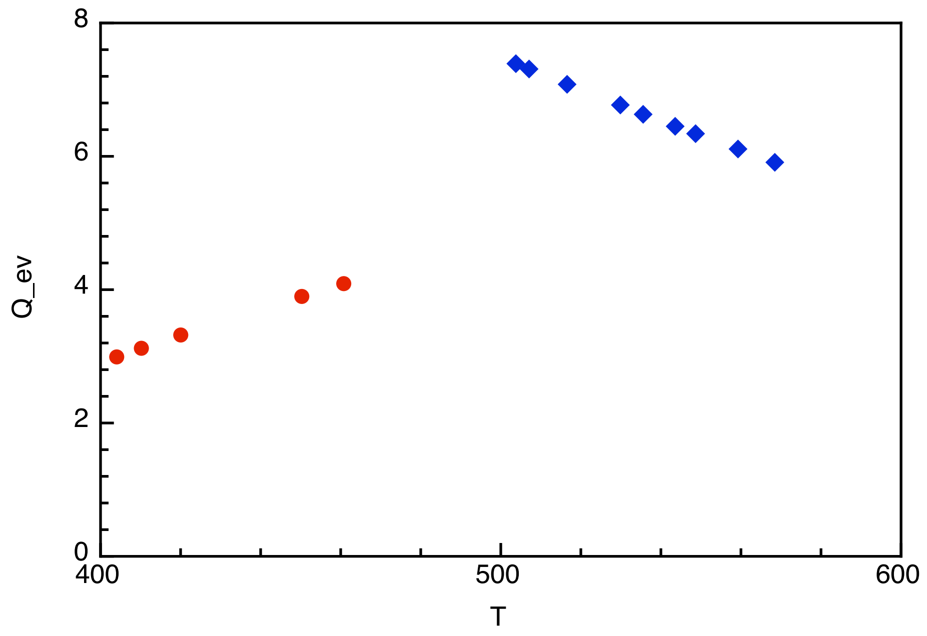

8
6
4
2
0
Q_ev
400
500
600
T


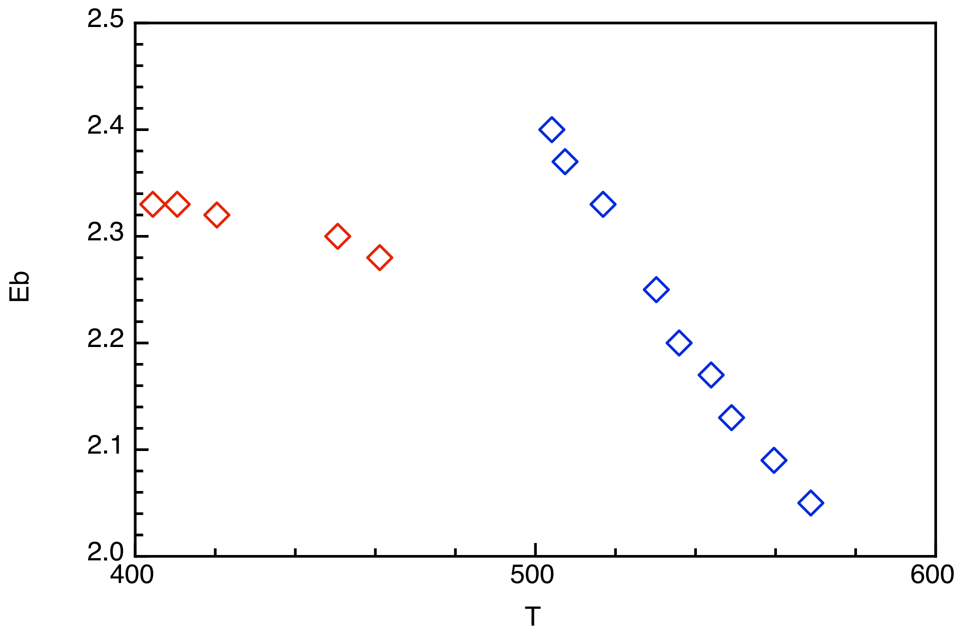

2.5
2.4
2.3
2.2
2.1
2.0
Eb
400
500
600
T

# Kawamura

K. Kawamura, et al., J. At, Energy Soc. Jpn., **13**, 27 (2014)

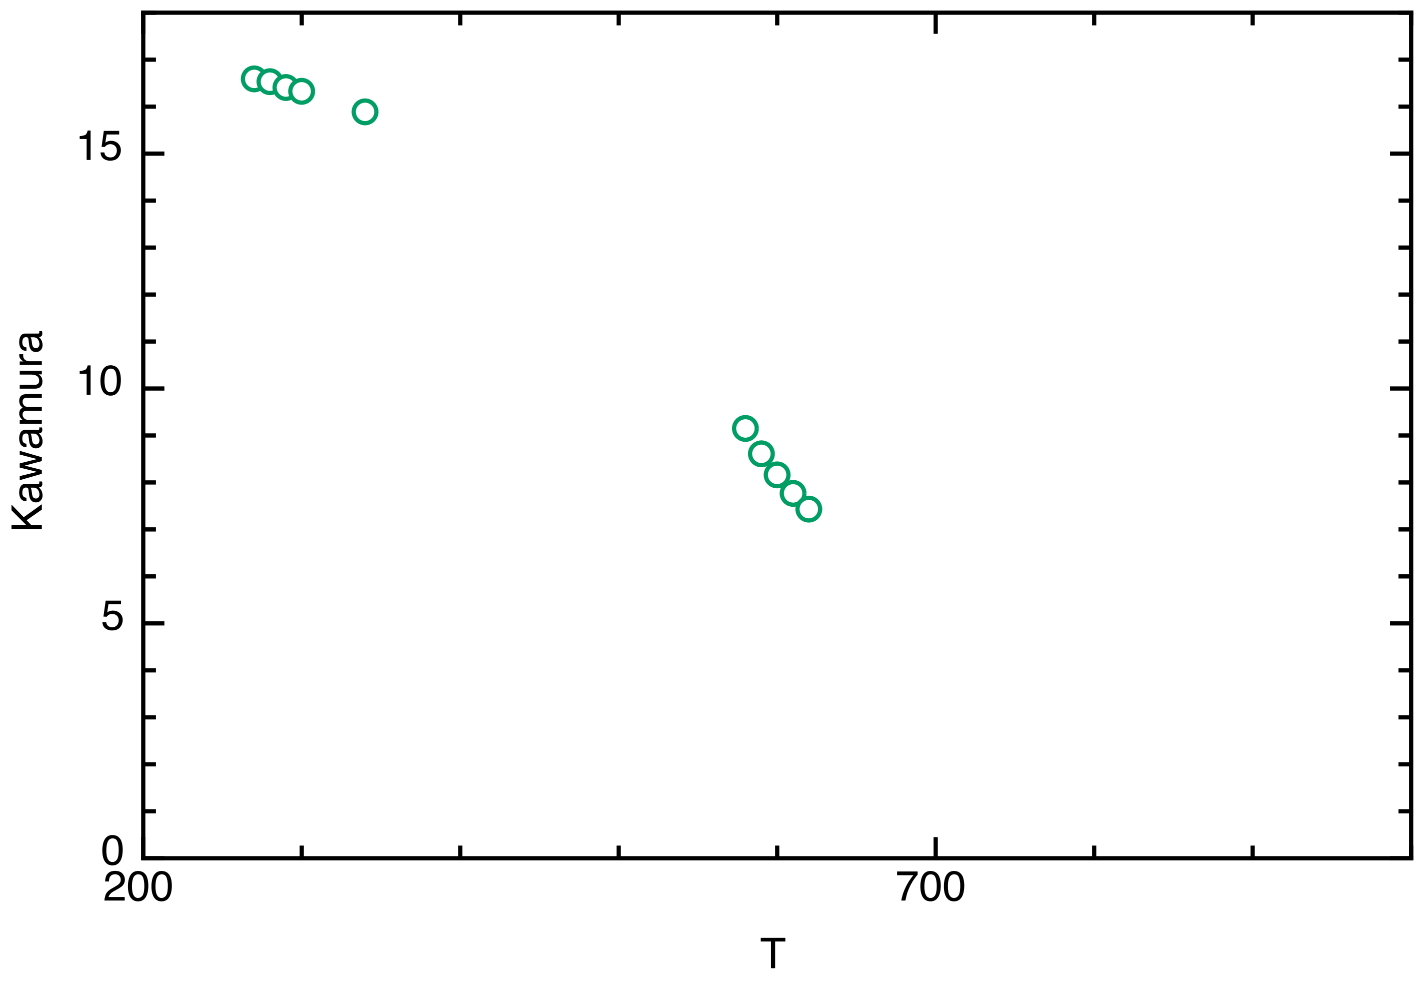

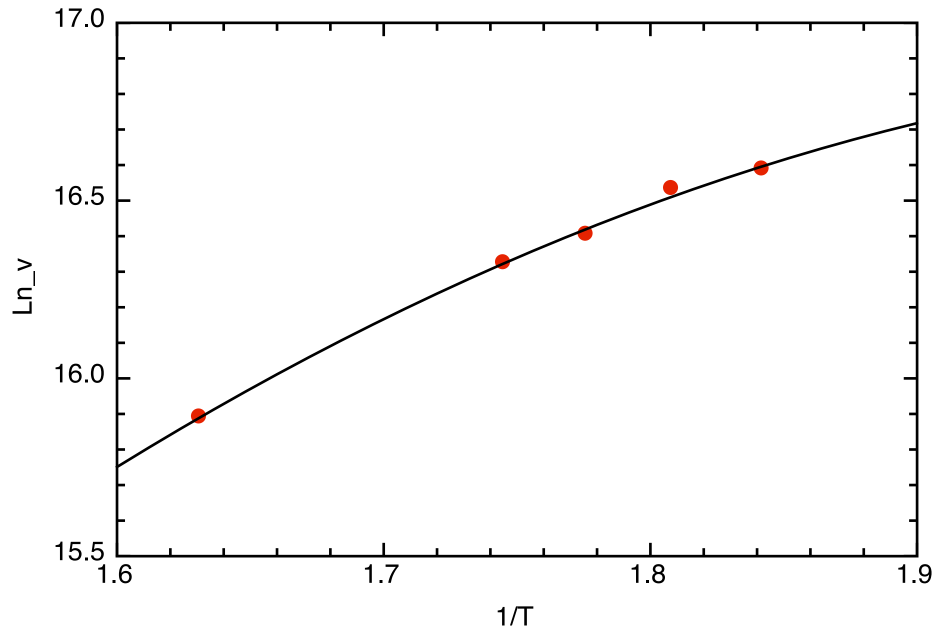


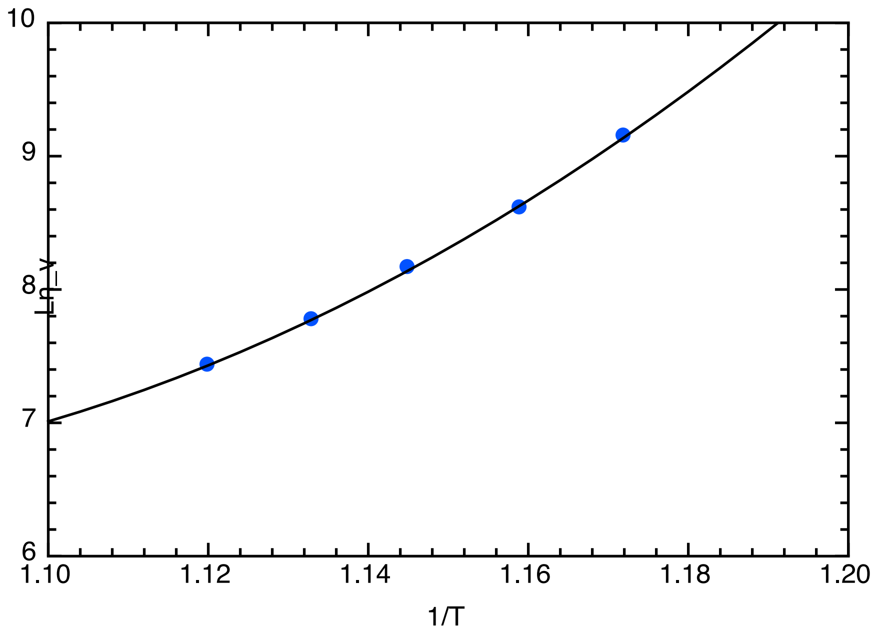


```
Iterations:   1
Seconds    :   5.7e-5
------------------------------------------
Chi squared          =      0.00080129

Parameters:                          Standard deviations:
deg     =      2.0000
const   =     -3.5978       Δconst =      5.8374
a1      =     19.5622       Δa1    =      6.7530
a2      =     -4.6683       Δa2    =      1.9498

Coefficient of Determination :            0.9974
Mean value of y-values y[i]  :            16.3480
Sum of squares of y[i]-yMean :            0.3048
Sum of squares of residuals  :            0.00080129
```

```
Fitted parameters:                   Standard deviations:
const   =      -2350.6759    Δconst =      4726.4824
a1      =       6301.0512    Δa1    =     12377.8859
a2      =      -5636.1528    Δa2    =     10803.8057
a3      =       1687.5705    Δa3    =      3142.8878

Fitted parameters:                   Standard deviations:
const   =       187.0352     Δconst =      43.7713
a1      =      -345.0459     Δa1    =      76.3976
a2      =       164.8972     Δa2    =      33.3286

Fitted parameters:                   Standard deviations:
const   =      -29.5089      Δconst =      1.7433
a1      =       32.9315      Δa1    =      1.5213
```

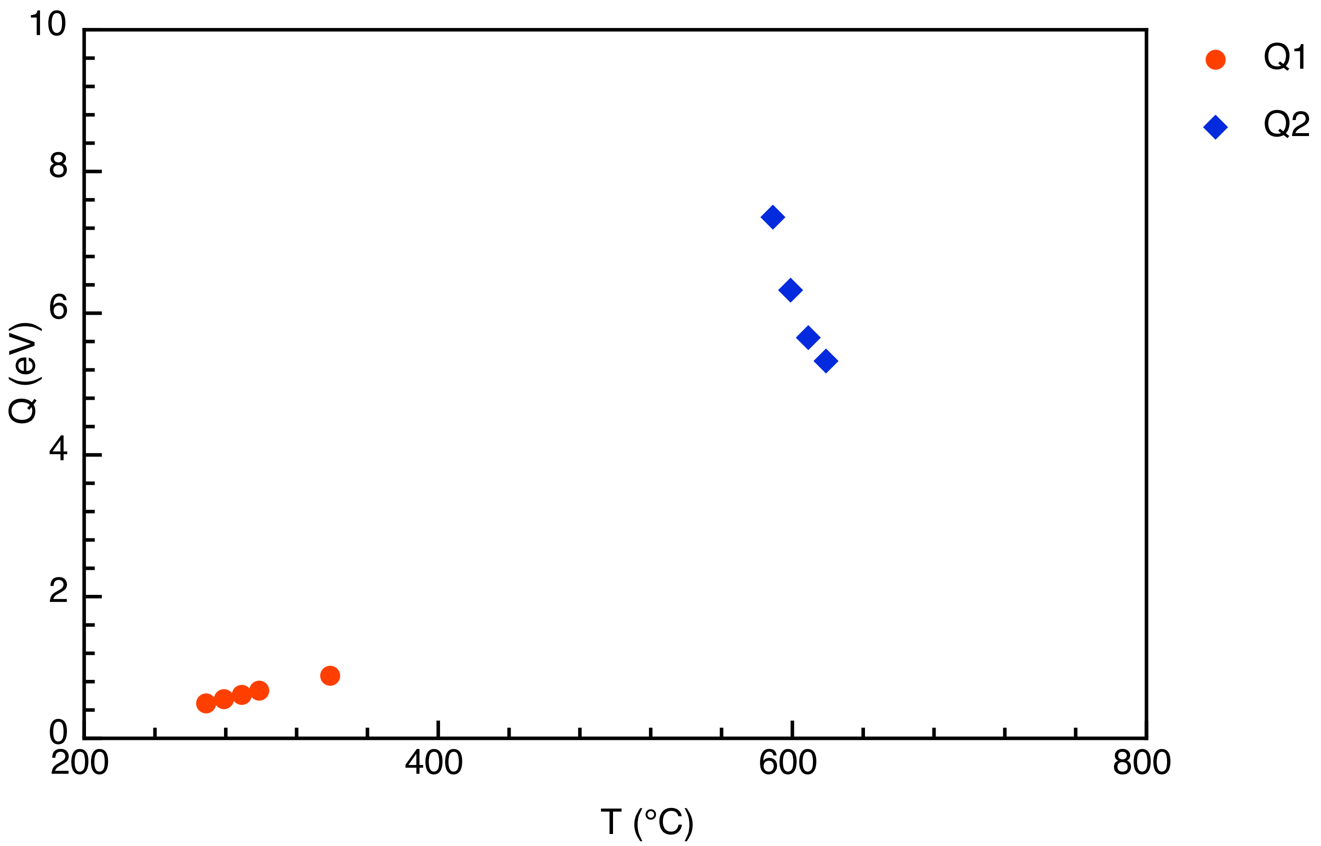
Q1
Q2
Q (eV)
T (°C)
0
2
4
6
8
10
200
400
600
800

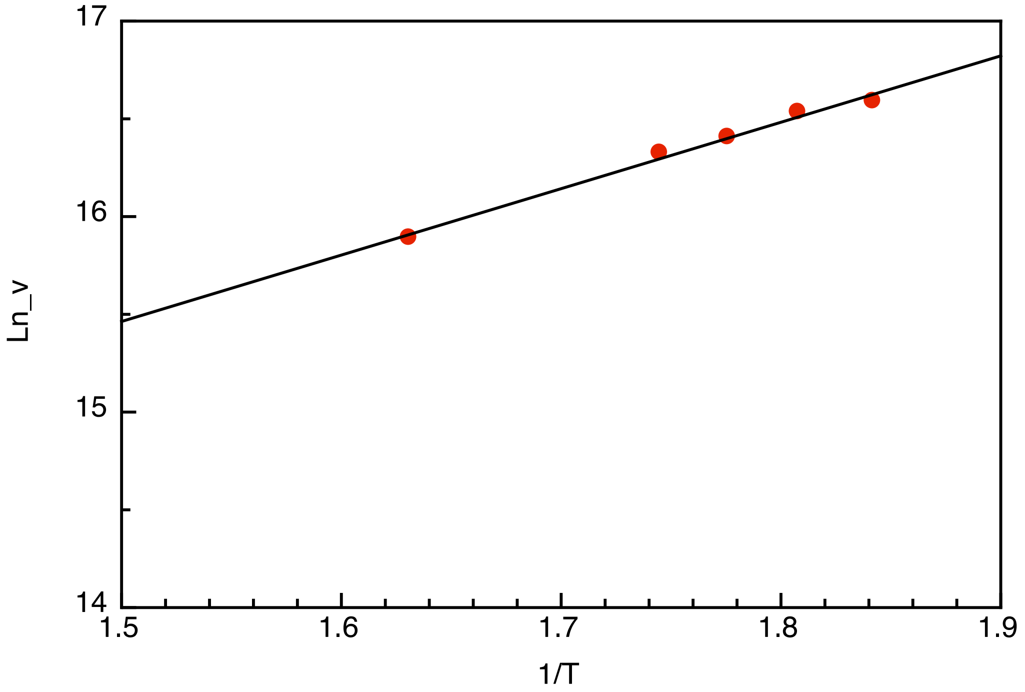


y = 10.36 + 3.40 x

y = log_{10}(v)

v = 2.29x10^(10) exp(2.3x(3.40x))

↓

Eb = 0.67 eV

```
Iterations:   1
Seconds    :  6.6e-5
------------------------------------------
Chi squared          =      0.0030979

Parameters:                       Standard deviations:
deg     =       1.0000
const   =      10.3685       Δconst =      0.3501
a1      =       3.3967       Δa1    =      0.1987

Correlation coefficient:      :           0.9949
Significance of correlation:  :           18.3320 %

Coefficient of Determination :            0.9898
Mean value of y-values y[i]  :            16.3480
Sum of squares of y[i]-yMean :            0.3048
Sum of squares of residuals  :            0.0030979
```

# B2O3

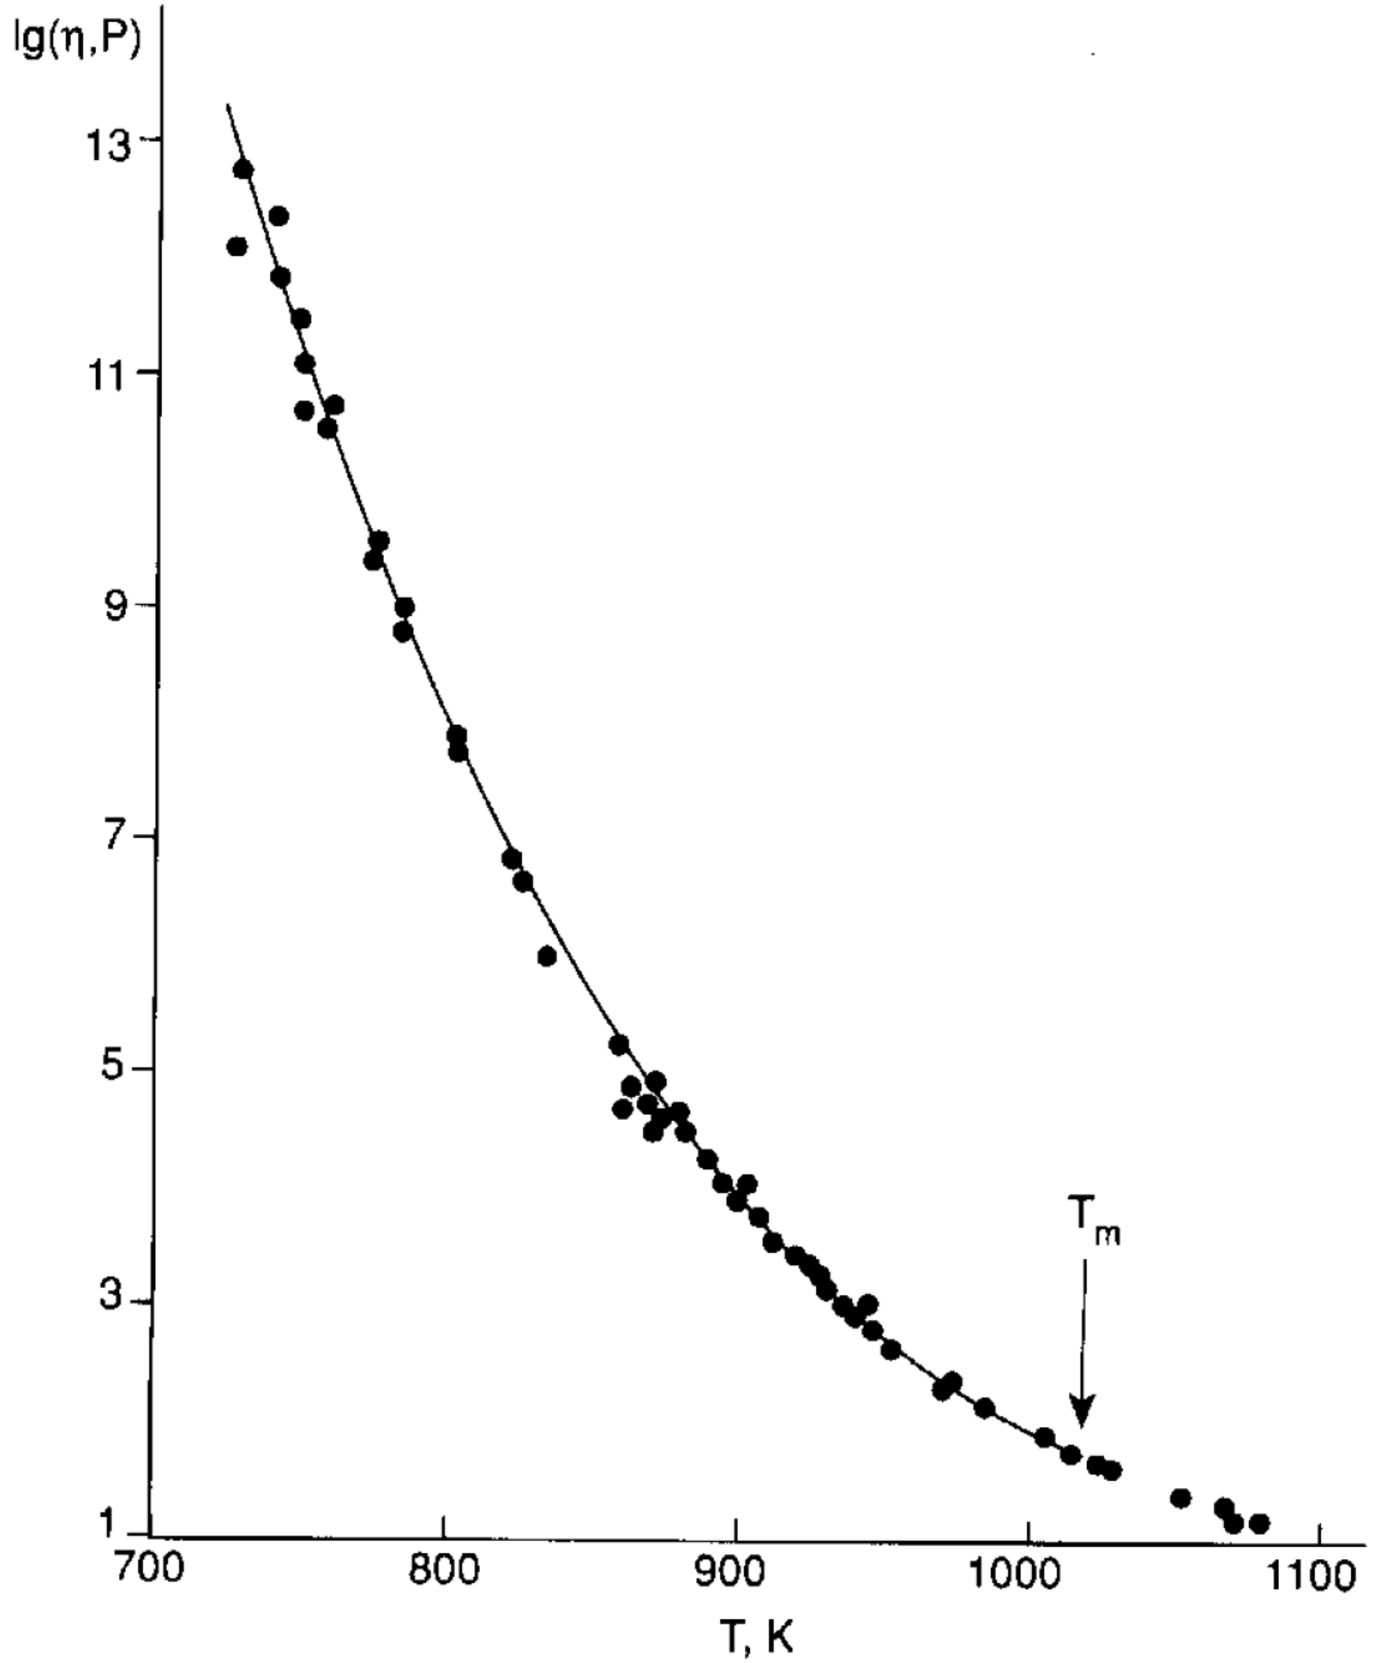


S.V. Nemilov, Thermodynamik and Kinetic Aspects of the Vitreous State, (CRC, 1995)

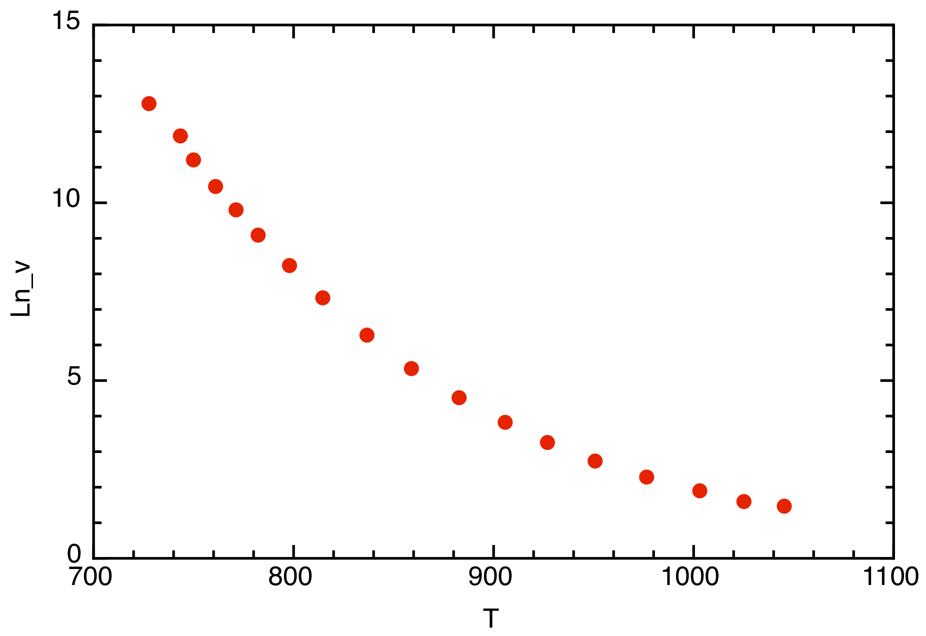
15
10
5
0
Ln_v
700
800
900
1000
1100
T

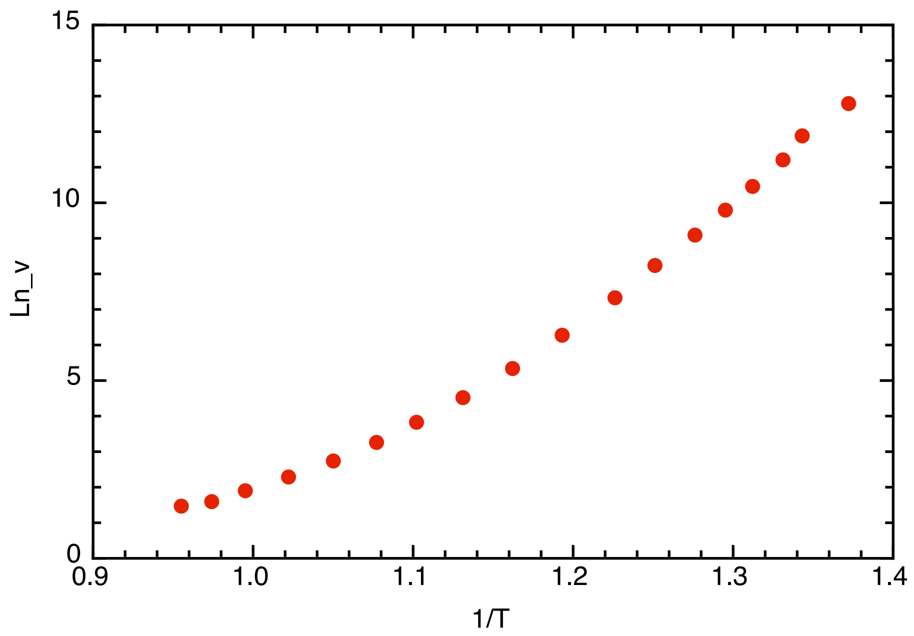
15
10
5
0
Ln_v
0.9
1.0
1.1
1.2
1.3
1.4
1/T

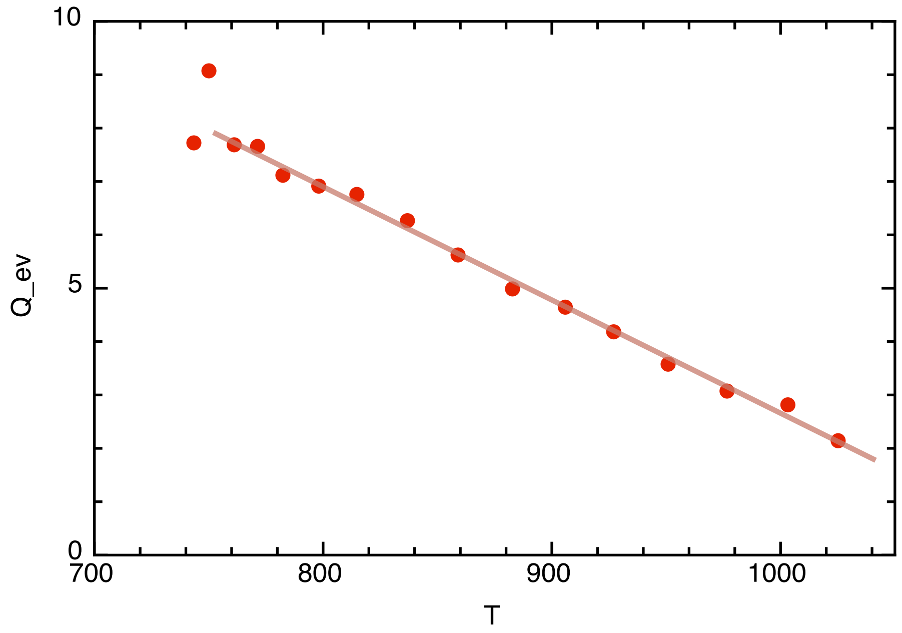
10
5
0
Q_ev
700
800
900
1000
T

# Glucose

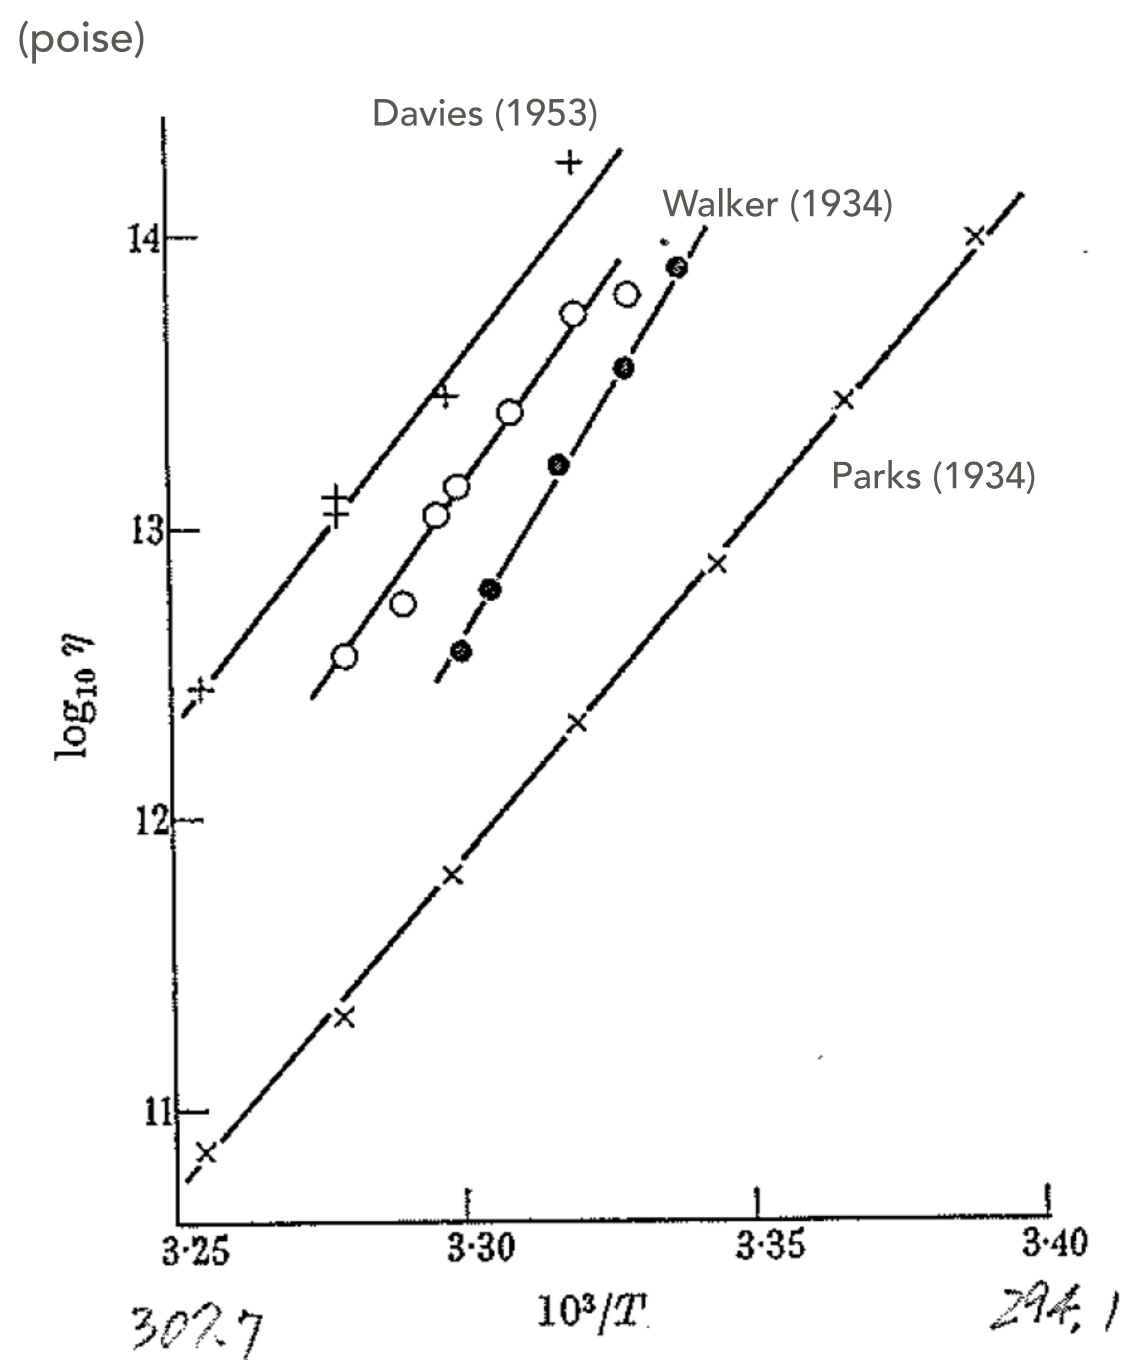


R. O. Davies and G. O. Jones, Proc. Roy. Soc. A**217**, 26 (1953)

Q = 125±10 kcal/mol

= 5.2 eV

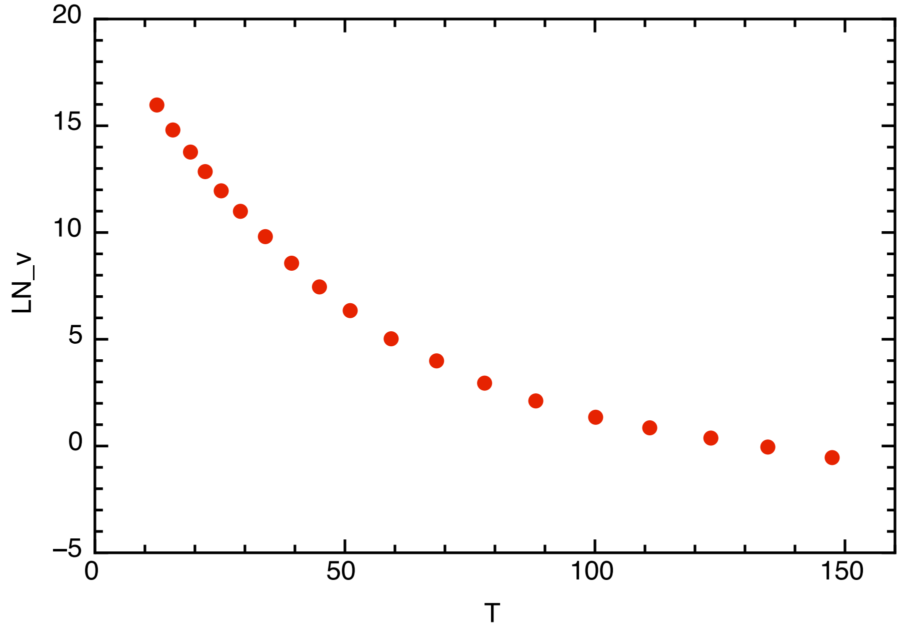

20
15
10
5
0
−5
LN_v
0
50
100
150
T


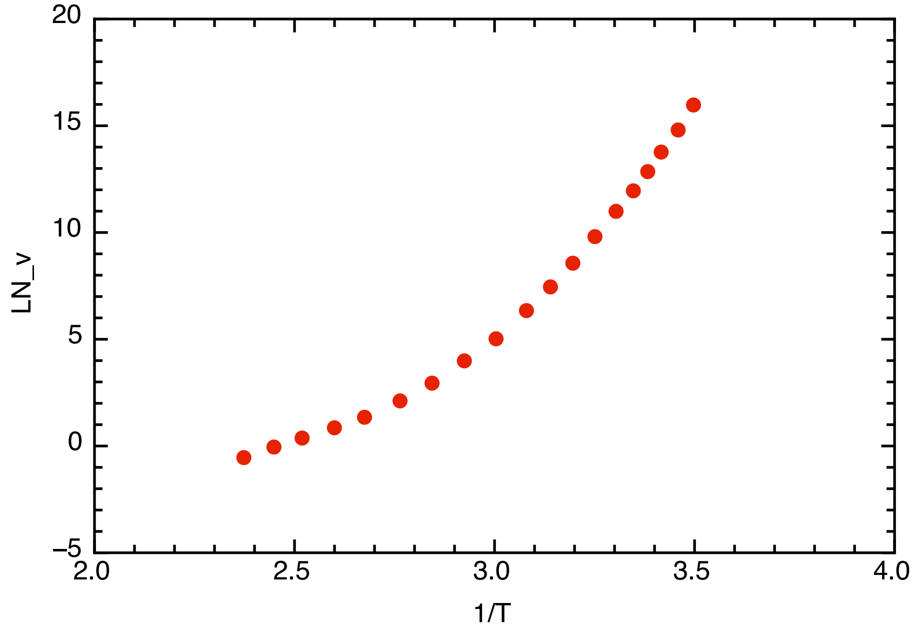

20
15
10
5
0
−5
LN_v
2.0
2.5
3.0
3.5
4.0
1/T


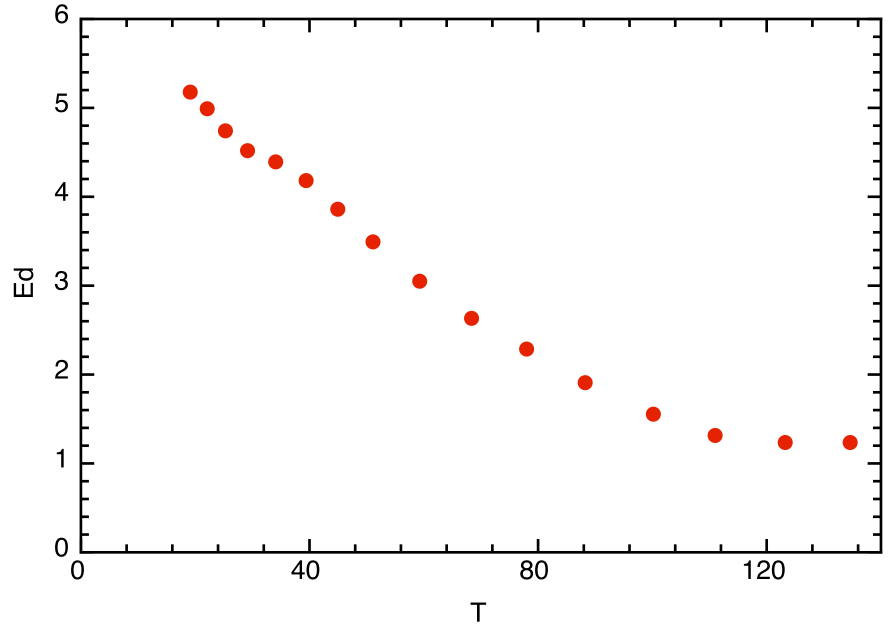

6
5
4
3
2
1
0
Ed
0
40
80
120
T

# Glycerol

J. Chem. Thermodyn. **113**, 162 (2017)
Abel G.M.Ferreira, Ana P.V.Egas, Isabel M.A.Fonseca, Ana C.Costa, Danielly C.Abreu, Lélio Q.Lobo

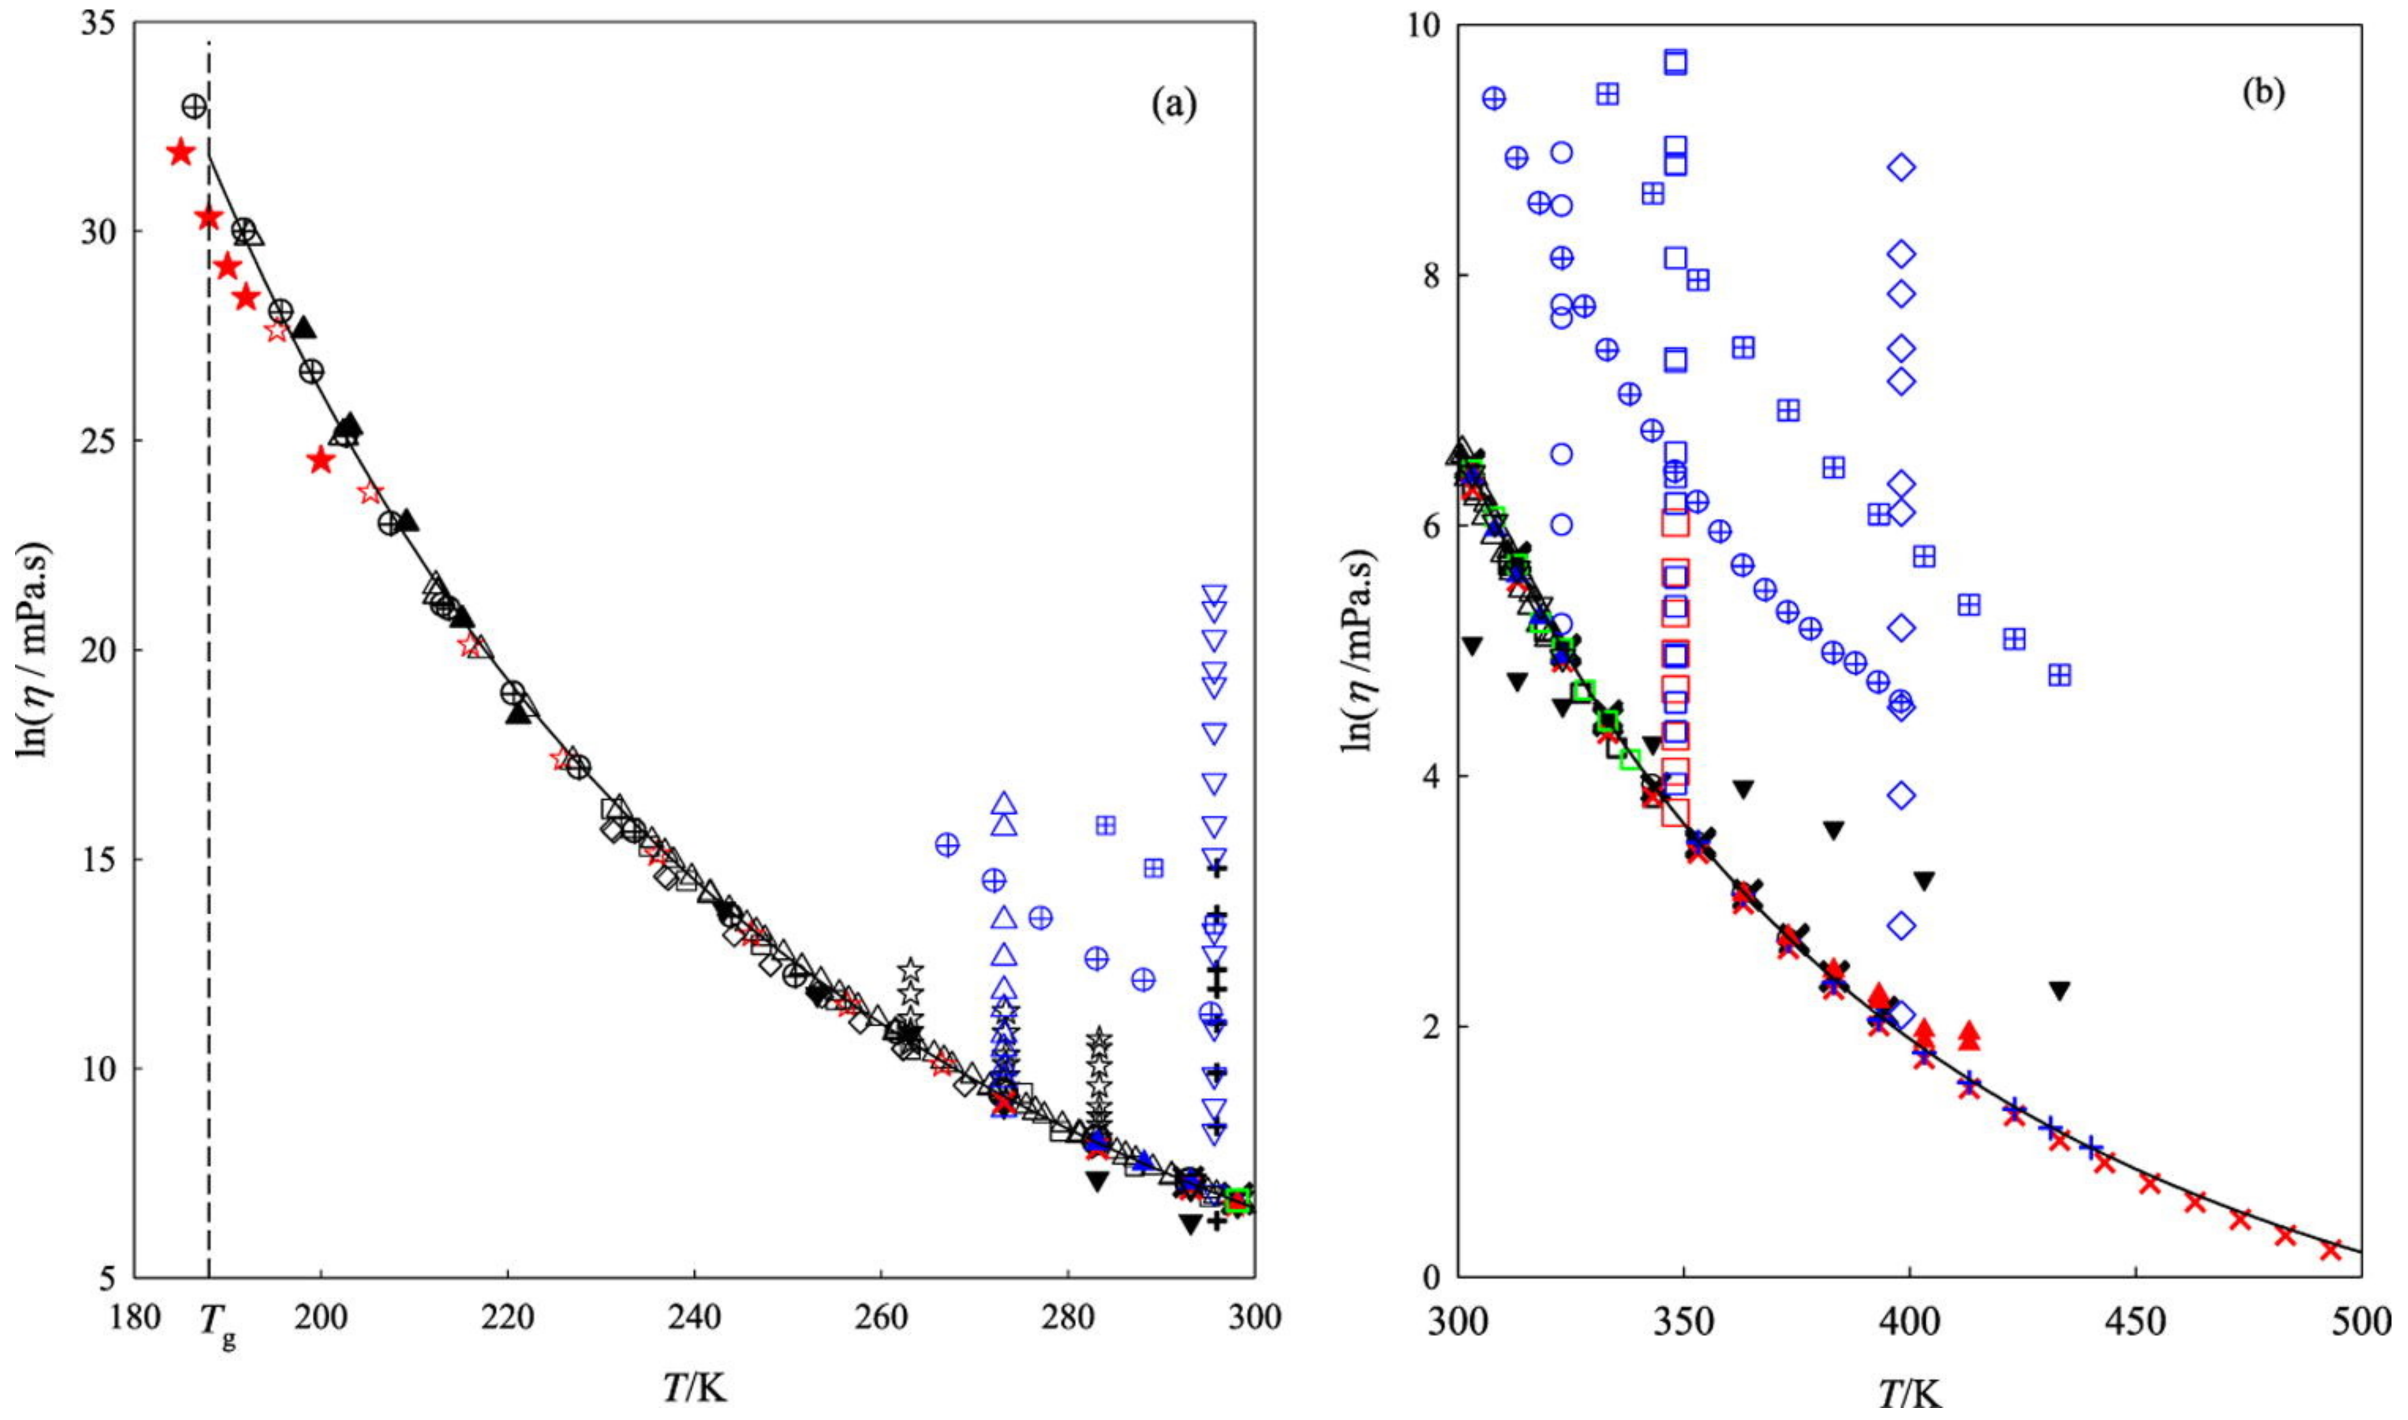

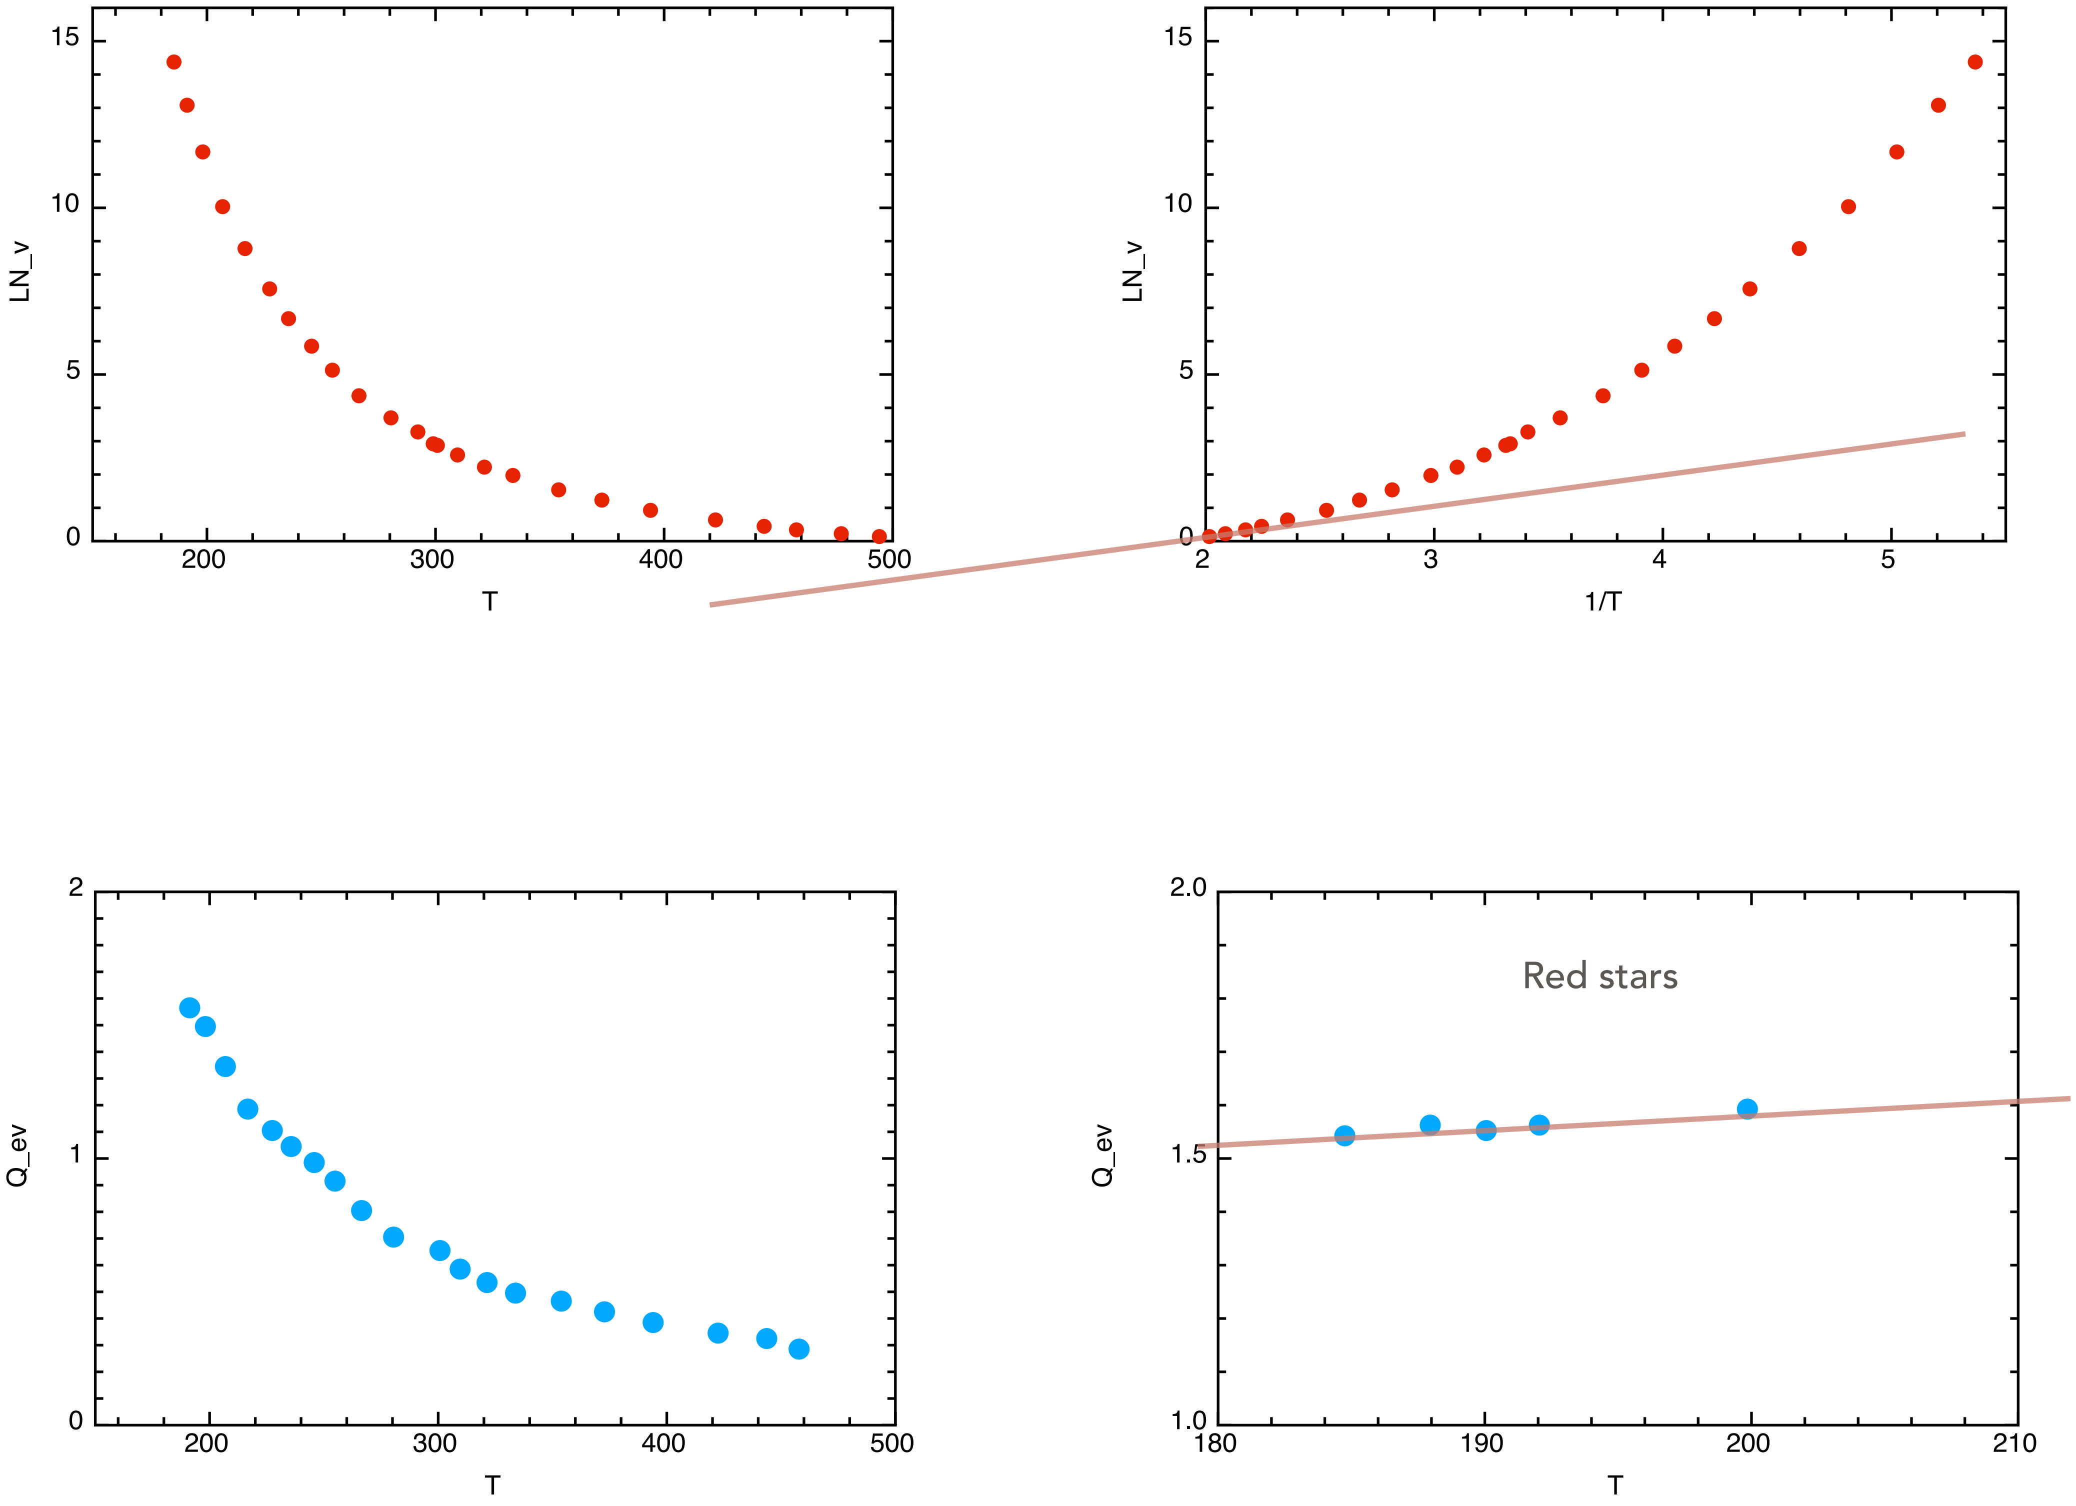
LN_v
T
LN_v
1/T
Q_ev
T
Q_ev
T
Red stars

# o-Terphenyl

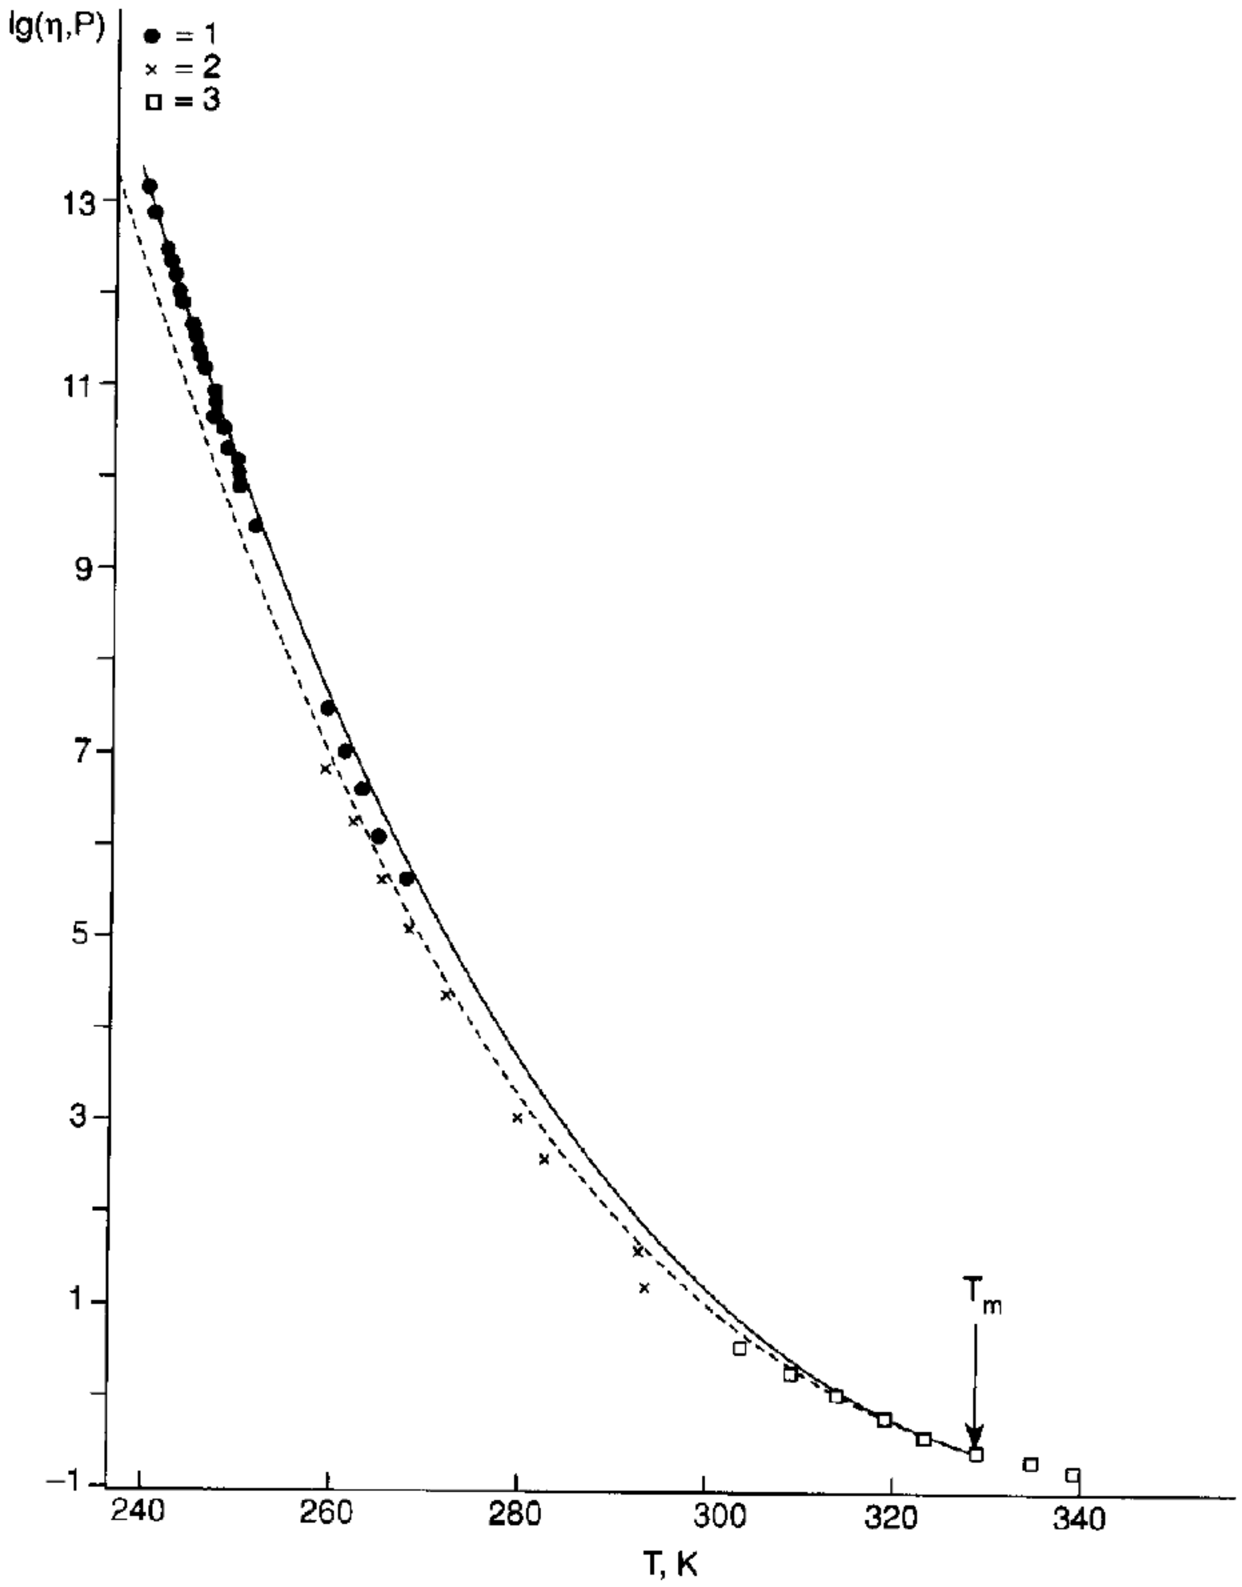


S.V. Nemilov, Thermodynamik and Kinetic Aspects of the Vitreous State, (CRC, 1995)

Valence-configurational theory (solid line)
Adam-Gibbs theory (dashed line)

S.S. Chang and A.B. Bestul, J. Chem. Phys. **56**, 503 (1972)


1) W.T. Laughlin, J. Phys. Chem. **76**, 2317 (1972)
2) R.J. Greet, J. Chem. Phys. **46**, 1243 (1967)
3) M. Cukierman, J. Chem. Phys. **59**, 3639 (1973)

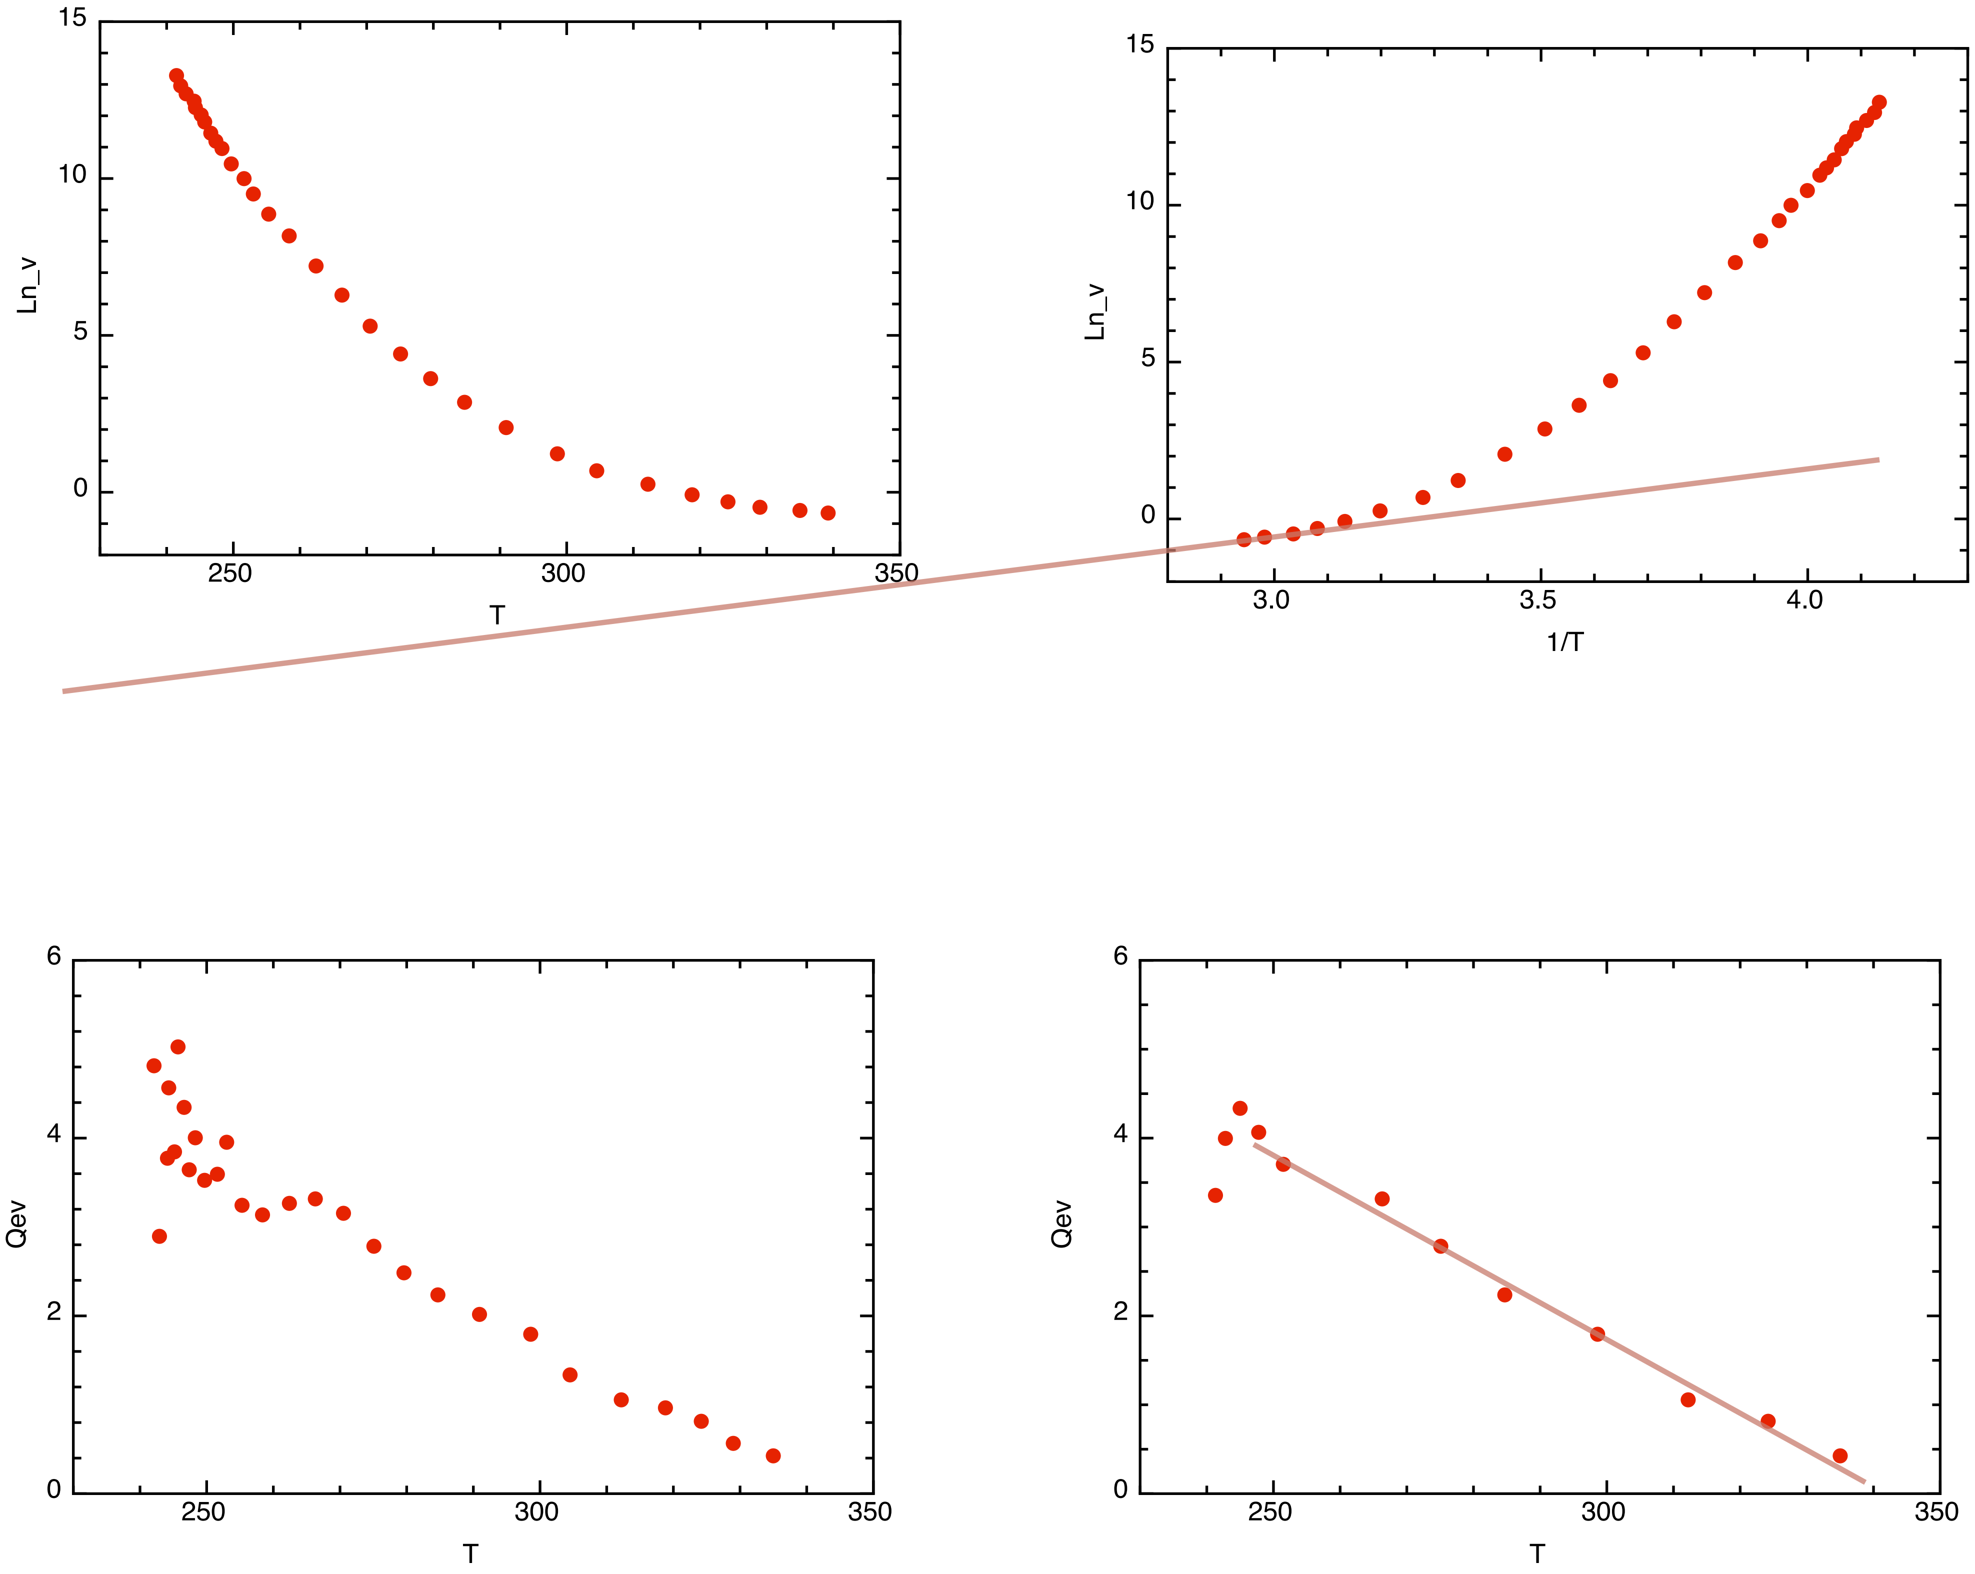

15
10
5
0
Ln_v
250
300
350
T
15
10
5
0
Ln_v
3.0
3.5
4.0
1/T
6
4
2
0
Qev
250
300
350
T
6
4
2
0
Qev
250
300
350
T

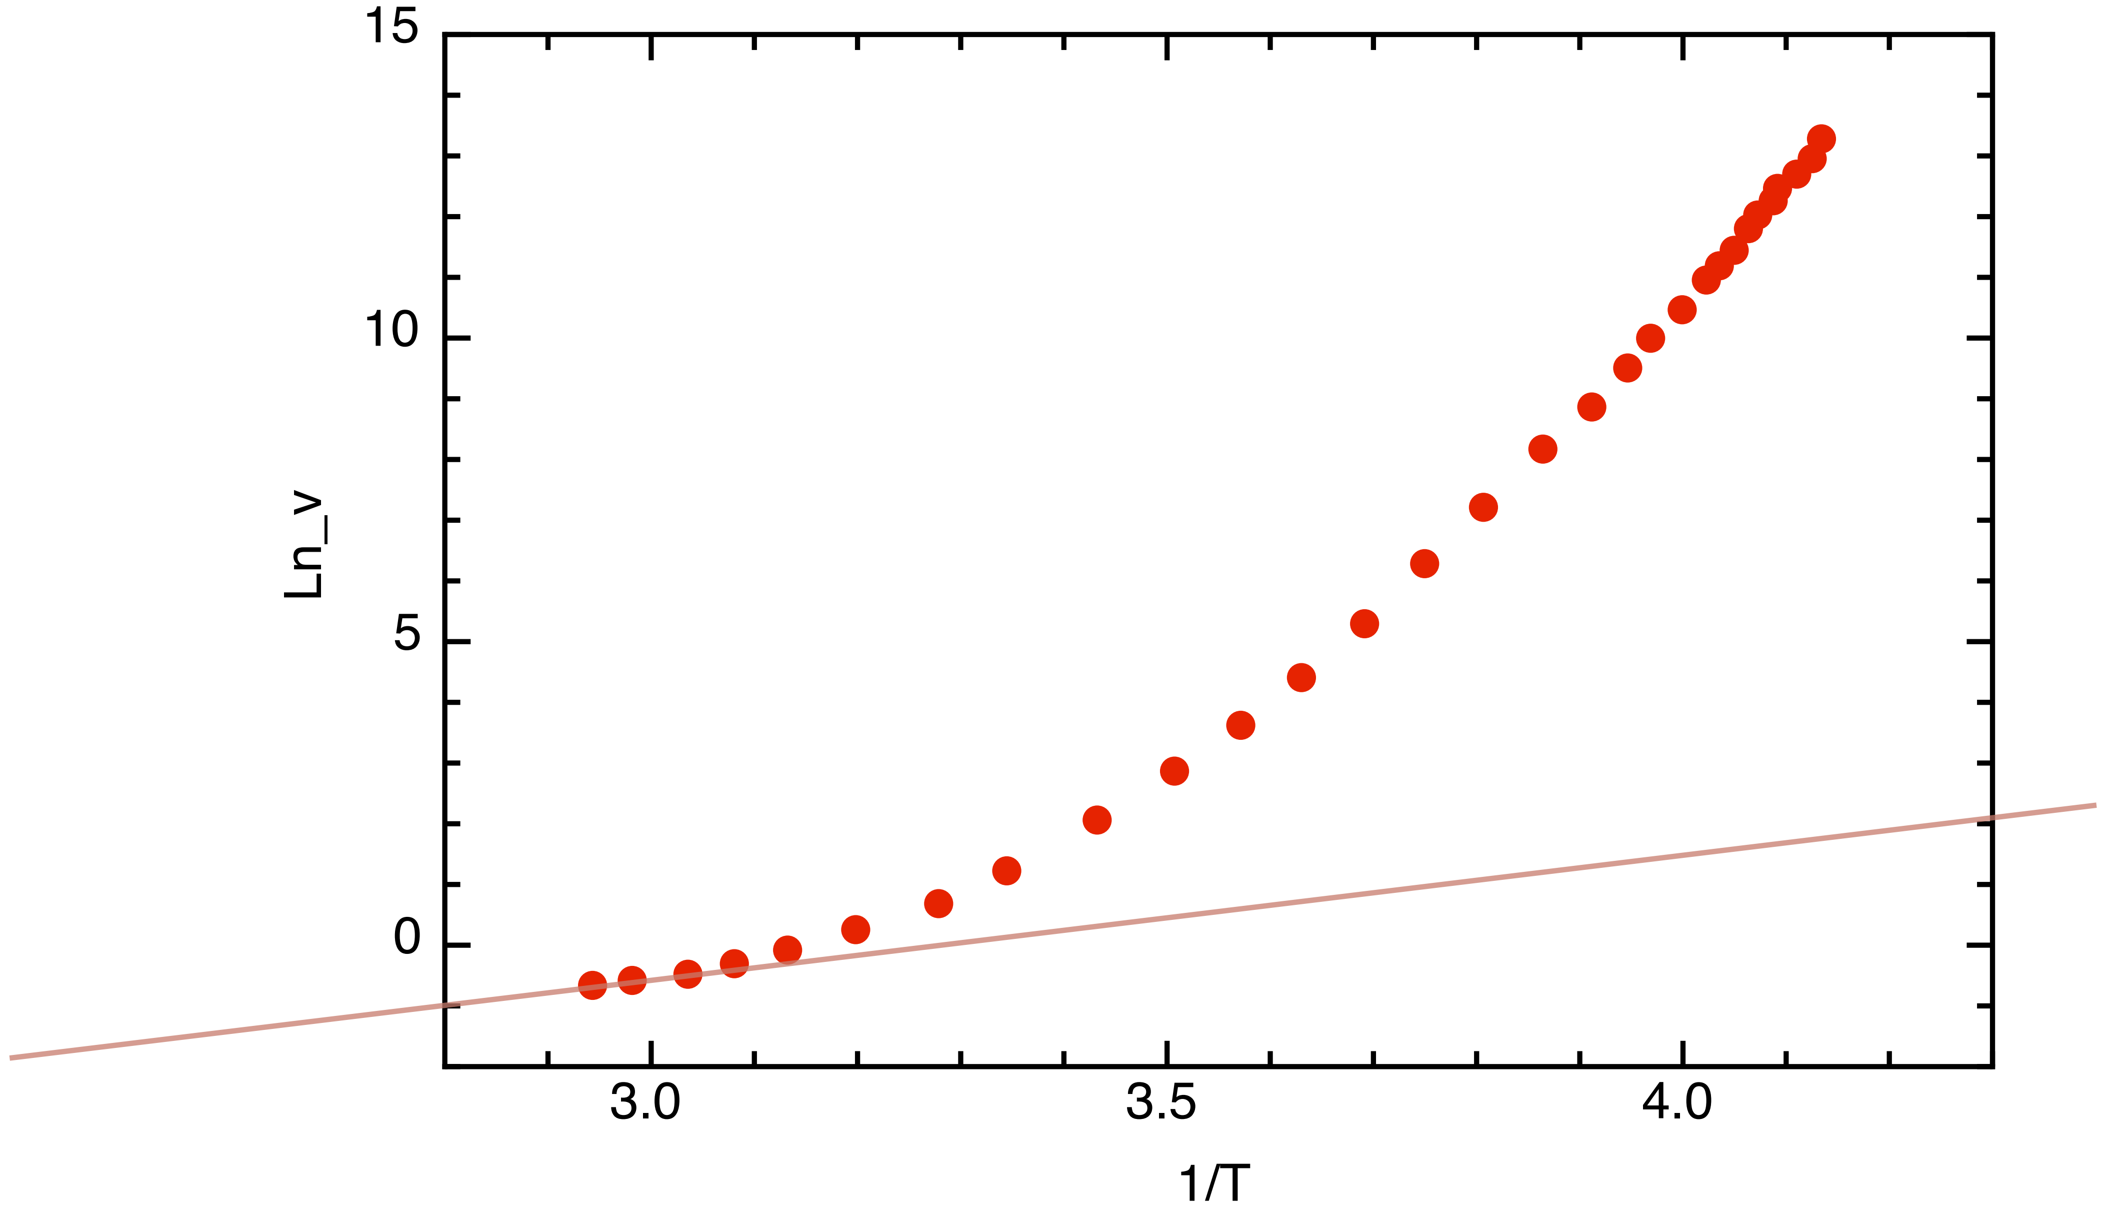


y = (3.0/1.5)(x-2.8)-1.0 = 2(x-2.8)-1

→ y_0 = -6.6

inacceptable

When y_0 = -3.5

at x = 3 y = 3.6x2.3/3 = 2.76 kK

= 0.24 eV

at x = 4.2 y = (13.5+3.5)x2.3/4.15 = 9.42 kK

= 0.81 eV

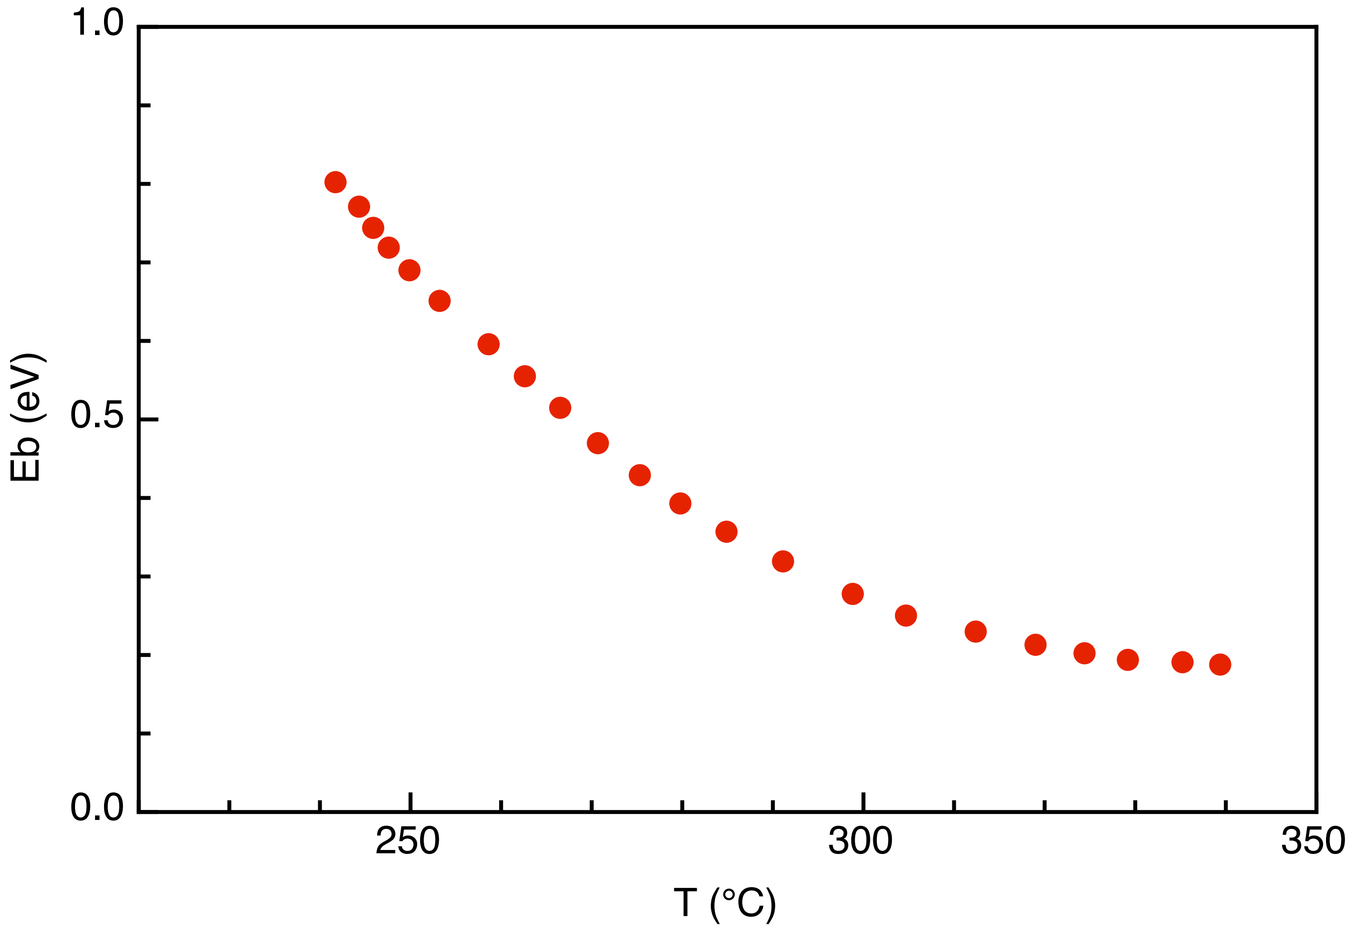
1.0
0.5
0.0
Eb (eV)
250
300
350
T (°C)

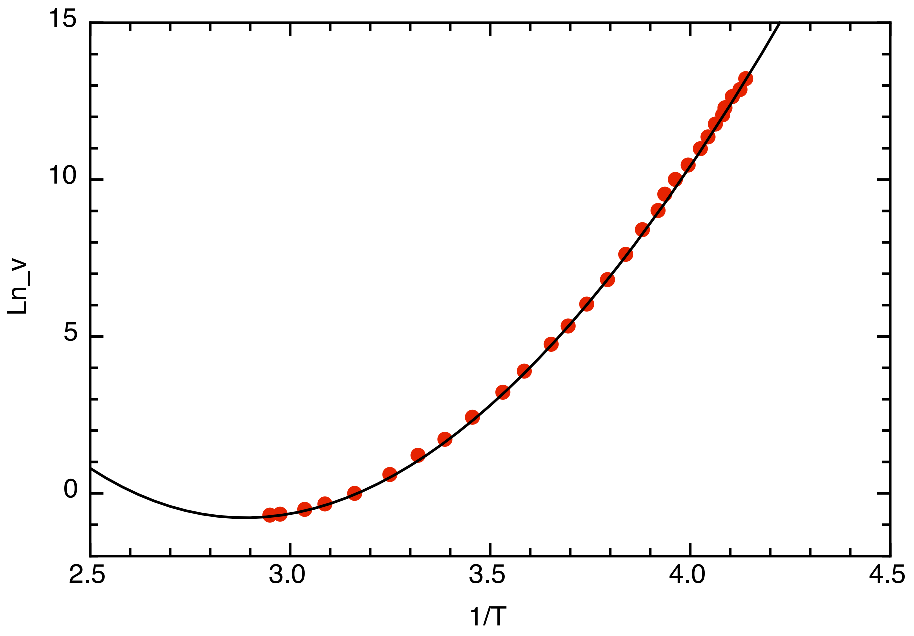


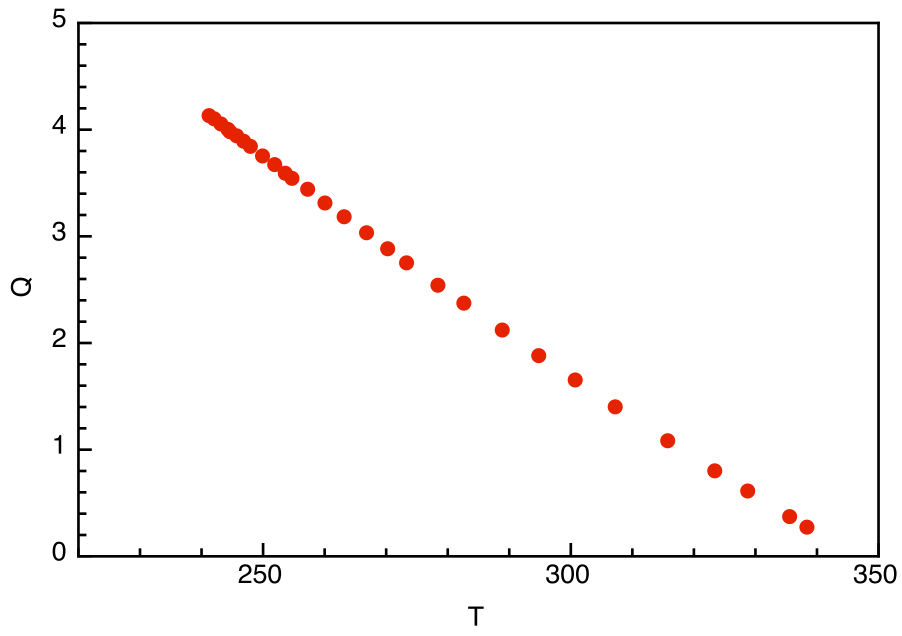


```
Iterations:    1
Seconds   :    2.7e-5
------------------------------------------
Chi squared          =    0.1379

Parameters:                  Standard deviations:
deg        =     3.0000
const      =   107.5910      Δconst     =    17.5140
a1         =   -83.3063      Δa1        =    14.9073
a2         =    18.7072      Δa2        =     4.2038
a3         =    -0.9885      Δa3        =     0.3929

Coefficient of Determination :          0.9998
Mean value of y-values y[i]  :          6.3728
Sum of squares of y[i]-yMean :          673.4242
Sum of squares of residuals  :          0.1379
```

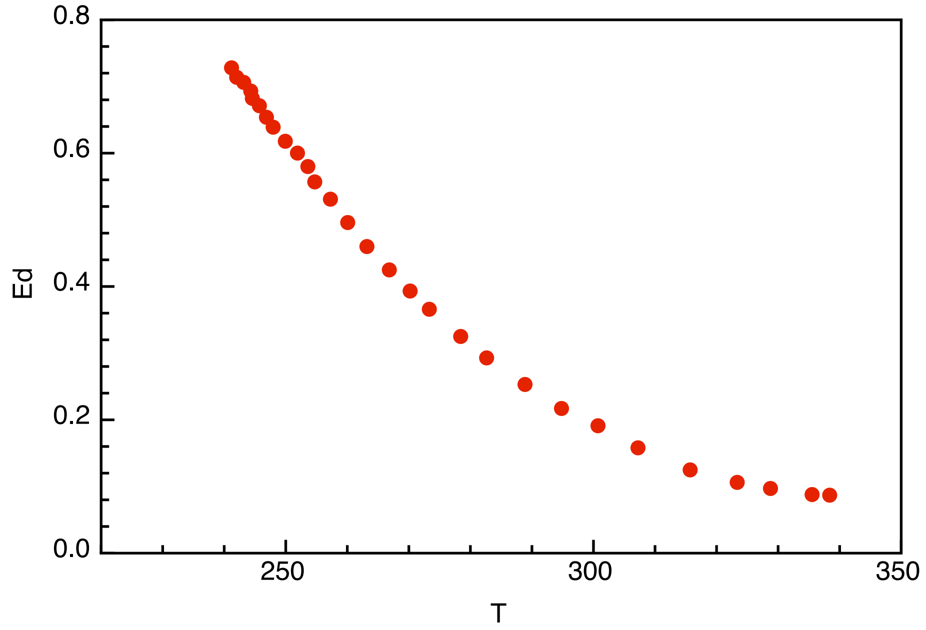

Supplement: Supplementary file 1 [file supplementals.pdf]
